# Supplementary material for: Electrochemical response of biological membranes to localized currents and external electric fields
Source: arXiv:2508.14001 ancillary file (2025-08-19)
Supplement: Supplementary file 1 [file Supplemental_material.pdf]

# Supplemental Material

## Electrochemical response of biological membranes to localized currents and external electric fields

Joshua B. Fernandes<sup>1,2</sup>, Hyeonjoo Row<sup>1,3</sup>, Kranthi K. Mandadapu<sup>1,2</sup>, and Karthik Shekhar<sup>1,3,4</sup>

<sup>1</sup> Department of Chemical and Biomolecular Engineering, University of California, Berkeley, CA 94720, USA

<sup>2</sup> Chemical Sciences Division, Lawrence Berkeley National Laboratory, CA 94720, USA

<sup>3</sup> Helen Wills Neuroscience Institute, California Institute for Quantitative Biosciences, QB3, Center for Computational Biology, University of California, Berkeley, CA 94720, USA

<sup>4</sup> Biological Systems Division, Lawrence Berkeley National Laboratory, Berkeley, CA 94720, USA

## Contents

|                                                                                                        |           |
|--------------------------------------------------------------------------------------------------------|-----------|
| <b>I. Nondimensionalization and linearized dynamics</b>                                                | <b>2</b>  |
| 1. Length, time, and speed scales . . . . .                                                            | 2         |
| 2. Governing equations . . . . .                                                                       | 3         |
| 3. Initial and boundary conditions . . . . .                                                           | 3         |
| <b>II. Linear superposition</b>                                                                        | <b>4</b>  |
| <b>III. Boundary layer theory</b>                                                                      | <b>5</b>  |
| 1. Bulk electrolyte . . . . .                                                                          | 5         |
| 2. Diffuse layer at the membrane surface . . . . .                                                     | 6         |
| 3. Diffuse layer at the electrode surface . . . . .                                                    | 8         |
| 4. Leading-order uniform solution . . . . .                                                            | 9         |
| <b>IV. Early time solution: Point-charge approximation</b>                                             | <b>9</b>  |
| <b>V. Late time solutions: Blocking electrodes</b>                                                     | <b>12</b> |
| 1. Near-field ( $r < L$ ) solution . . . . .                                                           | 14        |
| 2. Far-field, capacitive regime ( $r > L$ , $\tau_D < t < r/v$ ) . . . . .                             | 15        |
| 3. Far field, diffusive regime ( $r > L$ , $t > r/u$ ) . . . . .                                       | 17        |
| <b>VI. Late time solutions: Faradaic electrodes</b>                                                    | <b>18</b> |
| 1. Near-field ( $r < L$ ) solution . . . . .                                                           | 19        |
| 2. Far-field, capacitive regime ( $r > L$ , $\tau_D < t < r/v$ ) . . . . .                             | 21        |
| 3. Steady-state solution . . . . .                                                                     | 21        |
| <b>VII. External current</b>                                                                           | <b>22</b> |
| 1. Blocking electrodes ( $n_D = 4$ , $\hat{u} = (2 + \chi)^{-1}$ , $\hat{v} = 1 - \hat{u}$ ) . . . . . | 22        |
| (a). Contribution from $\bar{\phi}^C$ . . . . .                                                        | 22        |
| (b). Contribution from $\bar{\phi}^V$ . . . . .                                                        | 23        |
| (c). Linear superposition . . . . .                                                                    | 23        |
| 2. Ideal Faradaic electrode ( $n_D = 2$ , $\hat{u} = (1 + \chi)^{-1}$ , $\hat{v} = 1$ ) . . . . .      | 23        |
| (a). Contribution from $\bar{\phi}^C$ . . . . .                                                        | 24        |
| (b). External current to maintain the applied voltage . . . . .                                        | 24        |
| (c). Linear superposition . . . . .                                                                    | 24        |
| <b>References</b>                                                                                      | <b>24</b> |
| <b>A. Image charge transformations</b>                                                                 | <b>25</b> |
| <b>B. Hankel transforms of specific functions</b>                                                      | <b>27</b> |

This document is organized as follows. Section I presents the governing equations in dimensionless form. Section II exploits linearity to decompose the overall problem into a current-driven subproblem and a voltage-driven subproblem, and states the associated initial and boundary conditions. Section III formulates the boundary layer theory comprised of the outer bulk solution and the inner membrane- and electrode-side diffuse layer solutions. The outer and inner solutions are combined via asymptotic matching. Section IV uses a point-charge approximation to obtain closed-form expressions for the potential at early times in the electrostatic regime. Section V analyses the spatiotemporal electrochemical response for blocking electrodes, deriving the asymptotic formulas for the near-field, capacitive, and diffusive regimes presented in the main text. Section VI repeats the analysis for idealized Faradaic electrodes. Section VII coarse-grains the spatially resolved solutions to an equivalent lumped circuit and derives a global current voltage relationship for both electrode types. Two Appendices derive mathematical identities used in Secs. IV and V.

## I. Nondimensionalization and linearized dynamics

In this first section, we summarize characteristic scales featuring in the problem and then recast the linearized Poisson-Nernst-Planck (PNP) equations, and associated initial and boundary conditions, in dimensionless form. The resulting non-dimensional groups, in particular the small parameter  $\eta \equiv \lambda_D/L$  and the capacitance ratio  $\chi$ , will be used throughout this document.

### 1. Length, time, and speed scales

Three length scales control the coupled membrane-electrolyte system: the Debye screening length,  $\lambda_D \equiv \sqrt{\epsilon k_B T / (2C^0 e^2)}$ , which sets the thickness of every diffuse charge layer [1–3]; the membrane thickness  $\delta^M$ ; and the electrode-membrane gap  $L$ . In typical physiological settings  $\lambda_D, \delta^M \sim \mathcal{O}(\text{nm})$  whereas  $L$  can range from microns to millimeters. Hence  $L/\lambda_D, L/\delta^M \gg 1$ . These extreme separations justify the boundary-layer approach adopted in this work.

There are two natural diffusive timescales:  $\tau_D \equiv \lambda_D^2/D$ , governing local equilibration inside the diffuse charge screening layers, and the macroscopic diffusive time  $\tau_L \equiv L^2/D$ . Additionally, there are two  $RC$  timescales associated with diffuse charge dynamics in the system: the first is the bare electrolyte  $RC$  timescale  $\tau_B \equiv \lambda_D L/D$ , described in the work by Bazant et al., 2004 [3]. For electrode-membrane systems, we have recently identified a capacitive timescale,  $\tau_C \equiv \tau_B/(n_D/2 + \chi)$ , which is significantly smaller than  $\tau_B$  in typical scenarios [4] (see Table I in main text). Here,  $n_D$  is the number of diffuse charge layers in the system (four for blocking electrodes, two for perfect Faradaic electrodes),  $\chi \equiv \Gamma \delta^M / (2\lambda_D)$  is the ratio of the diffuse layer capacitance to twice the membrane capacitance, and  $\Gamma \equiv \epsilon/\epsilon^M$  is the ratio of permittivities of the electrolyte and the membrane. Finally, there is another macroscopic diffusional timescale  $\tau'_L \equiv L^2/D_{\text{eff}}$  associated with the late-time, radial spreading of charge through the confined electrolyte solution under sustained transmembrane ionic current. The effective radial diffusivity  $D_{\text{eff}} = ((1 + \chi)/(n_D/2 + \chi))(L/\lambda_D)D$  is identified in the main text.

Certain combinations of the length and time scales define speed scales that, as we shall see, will play important roles in the overall charge reorganization dynamics of our system. Combining the microscopic length  $\lambda_D$  with the microscopic time  $\tau_D$  gives a speed scale

$$u \equiv \frac{\lambda_D}{\tau_D} . \quad (\text{S.1})$$

On the other hand, electrochemical signals generated by a transmembrane ionic current propagate along the membrane surface with speed [5]

$$v \equiv (1 + \chi) \frac{\lambda_D}{\tau_D} . \quad (\text{S.2})$$

Thus  $u \equiv v/(1 + \chi)$ . In the following section, we nondimensionalize lengths by  $L$  and times by  $\tau_C$ . The nondimensional speeds are

$$\hat{v} \equiv \frac{v}{L/\tau_C} = \frac{1 + \chi}{n_D/2 + \chi} = \begin{cases} \frac{1 + \chi}{2 + \chi} & (\text{blocking}) \\ 1 & (\text{Faradaic}) \end{cases} , \quad (\text{S.3})$$

$$\hat{u} \equiv \frac{u}{L/\tau_C} = \frac{1}{n_D/2 + \chi} = \begin{cases} \frac{1}{2 + \chi} & \text{(blocking)} \\ \frac{1}{1 + \chi} & \text{(Faradaic)} \end{cases}, \quad (\text{S.4})$$

where the rightmost expressions are obtained by using  $n_D = 4$  for blocking electrodes, and  $n_D = 2$  for ideal Faradaic electrodes.

## 2. Governing equations

As explained in the main text, the concentration changes produced by transmembrane ionic currents and physiologically relevant voltages are small, so a linear approximation is valid. The resulting linearized equations for the total ion concentration and charge density, written in dimensionless form, are

$$\frac{\partial \bar{C}}{\partial \hat{t}} + \hat{\nabla} \cdot \bar{\mathbf{j}}_C = 0, \quad \bar{\mathbf{j}}_C = -\frac{\eta}{n_D/2 + \chi} \hat{\nabla} \bar{C}, \quad (\text{S.5})$$

$$\frac{\partial \bar{\rho}}{\partial \hat{t}} + \hat{\nabla} \cdot \bar{\mathbf{j}}_\rho = 0, \quad \bar{\mathbf{j}}_\rho = -\frac{\eta}{n_D/2 + \chi} (\hat{\nabla} \bar{\rho} + \hat{\nabla} \bar{\phi}), \quad (\text{S.6})$$

$$-\eta^2 \hat{\nabla}^2 \bar{\phi} = \bar{\rho}, \quad (\text{S.7})$$

where  $\hat{\nabla} \equiv \partial/\partial \hat{\mathbf{x}}$ ,  $\hat{\mathbf{x}} \equiv \mathbf{x}/L$ ,  $\hat{t} \equiv t/\tau_C$ ,  $\eta \equiv \lambda_D/L$ ,  $\bar{\rho} \equiv (C_+ - C_-)/(2C^0)$  is the dimensionless charge density,  $\bar{C} \equiv (C_+ + C_- - 2C^0)/(2C^0)$  is the dimensionless disturbance in salt concentration, and  $\bar{\phi} \equiv \phi/\phi_T$  is the dimensionless electric potential. Here, we chose the initial salt concentration  $2C^0$  and thermal voltage  $\phi_T = k_B T/e$  as scales for the concentrations and electric potential, where  $k_B T$  is the thermal energy and  $e$  is the fundamental charge. Table S1 lists each dimensional symbol alongside its dimensionless counterpart.

The linearized equations (S.5)-(S.7) are also called the Debye-Falkenhagen equations [6]. Owing to linearization, salt and charge evolutions decouple; only the second and third equations for charge and potential will therefore be pursued, where the salt disturbance follows the usual diffusion equation.

Table S1: The dimensional quantities and their corresponding nondimensionalizations.

| Quantity             | Symbol            | Nondimensionalization                                                         |
|----------------------|-------------------|-------------------------------------------------------------------------------|
| Position             | $\mathbf{x}$      | $\hat{\mathbf{x}} = \mathbf{x}/L$ , $\bar{\mathbf{x}} = \mathbf{x}/\lambda_D$ |
| Time                 | $t$               | $\hat{t} = t/\tau_C$ , $\bar{t} = t/\tau_D$                                   |
| Salt concentration   | $C$               | $\bar{C} = C/(2C_0)$                                                          |
| Charge density       | $\rho$            | $\bar{\rho} = \rho/(2eC_0)$                                                   |
| Electric potential   | $\phi$            | $\bar{\phi} = \phi/\phi_T$                                                    |
| Salt flux            | $\mathbf{j}_C$    | $\bar{\mathbf{j}}_C = \mathbf{j}_C/(2C_0 L/\tau_C)$                           |
| Current flux         | $\mathbf{j}_\rho$ | $\bar{\mathbf{j}}_\rho = \mathbf{j}_\rho/(2eC_0 L/\tau_C)$                    |
| Areal charge density | $\sigma$          | $\bar{\sigma} = \sigma/(2eC_0 \lambda_D)$                                     |
| Imposed current      | $I$               | $\bar{I} = I/(\phi_T L g)$                                                    |
| Speed                | $v$               | $\hat{v} = v/(L/\tau_C)$                                                      |
| Speed                | $u$               | $\hat{u} = u/(L/\tau_C)$                                                      |

## 3. Initial and boundary conditions

The electrolyte is initially homogeneous:

$$\bar{\rho}(\hat{\mathbf{x}}, \hat{t} = 0) = 0. \quad (\text{S.8})$$

At the membrane surface  $z = 0$ , a circular patch of radius  $R^P$  delivers a uniform cationic current density  $I$ . The membrane is impermeable at all other locations. In dimensionless form at  $\hat{z} = 0$  (see Table S1),

$$\bar{\mathbf{j}}_\rho \cdot \mathbf{e}_z = \frac{\eta \bar{I}}{n_D/2 + \chi} \frac{\Theta(\hat{R}^P - \hat{r})}{\pi(\hat{R}^P)^2} \approx \frac{\eta \bar{I}}{n_D/2 + \chi} \frac{\delta(\hat{r})}{2\pi \hat{r}}, \quad (\text{S.9})$$

$$\bar{\phi} = \eta\chi \frac{\partial \bar{\phi}}{\partial \tilde{z}}, \quad (\text{S.10})$$

where  $\Theta$  is the Heaviside step function,  $\bar{I} = I/(\phi_{\text{T}} L g)$ , and  $\hat{R}^{\text{P}} \equiv R^{\text{P}}/L$ , where  $g \equiv \epsilon/\tau_{\text{D}}$  is the electrolyte conductivity. The charge dynamics in the vicinity of the transporter remains unperturbed by the presence of the electrodes and the ensuing dynamics has been explored in Ref. [5]. We therefore restrict attention to the regime  $\hat{r} \gg \hat{R}^{\text{P}} \sim \mathcal{O}(\hat{\lambda}_{\text{D}})$ . At such distances from the pore, the finite-sized ionic current can be approximated as if it were emitted from a point source. Accordingly, the Heaviside step function may be replaced by a delta function at  $\hat{r} = 0$ , as expressed in Eq.(S.9). Equation (S.10) is a Robin-type boundary condition that decouples the electrostatics in the electrolyte from the membrane. To quickly see how this condition arises, we write the Laplace equation within the membrane, i.e. Eq. (2) in the main text, in nondimensional form:

$$\frac{\partial^2 \bar{\phi}^{\text{M}}}{\partial \tilde{z}^2} + \left( \frac{\delta^{\text{M}}}{L} \right)^2 \frac{\partial^2 \bar{\phi}^{\text{M}}}{\partial \tilde{r}^2} = 0, \quad (\text{S.11})$$

where  $\tilde{z} \equiv z/\delta^{\text{M}}$  is the axial coordinate scaled by the membrane thickness, the length scale relevant for axial variations inside the membrane. Since  $\delta^{\text{M}}/L \ll 1$ , the radial term is much smaller than the axial term, so that  $\partial^2 \bar{\phi}^{\text{M}}/\partial \tilde{z}^2 \approx 0$ . Consequently,  $\bar{\phi}^{\text{M}}$  is linear with  $z$  inside the membrane. This, combined with the symmetry condition that  $\bar{\phi}^{\text{M}} = 0$  at the membrane midplane and the continuity conditions at the membrane surfaces (Eq. (3), main text), yields Eq. (S.10).

At the electrode surface  $\tilde{z} = 1$ , the applied potential imposes a Dirichlet condition:

$$\bar{\phi} = \bar{V}, \quad (\text{S.12})$$

where  $\bar{V} = V/\phi_{\text{T}}$ . For electrode kinetics, we treat two idealized cases:

- **Blocking electrodes** (no Faradaic reactions):

$$\bar{\mathbf{j}}_{\rho} \cdot \mathbf{e}_z = 0, \quad (\text{S.13})$$

giving  $n_{\text{D}} = 4$  diffuse layers, two on the membrane surfaces and two on the electrode surfaces.

- **Perfect Faradaic electrodes:**

$$\bar{\rho} = 0, \quad (\text{S.14})$$

so only the two membrane-side diffuse layers develop, giving  $n_{\text{D}} = 2$ .

## II. Linear superposition

The governing equations (S.6) and (S.7) are linear, so the full solution may be written as a superposition of two independent subproblems: (a) an imposed transmembrane ionic current with electrode potentials maintained at  $\bar{\phi} = 0$  and (b) an applied voltage of  $2\bar{V}$  across a completely impermeable membrane.

We pose a linear decomposition of the solutions:

$$\bar{\rho} = \bar{\rho}^{\text{C}} + \bar{\rho}^{\text{V}}, \quad (\text{S.15a})$$

$$\bar{\phi} = \bar{\phi}^{\text{C}} + \bar{\phi}^{\text{V}}, \quad (\text{S.15b})$$

where the superscripts ‘C’ and ‘V’ denote the *current-driven* and *voltage-driven* problems, respectively. The governing equations of the current problem are

$$\frac{\partial \bar{\rho}^{\text{C}}}{\partial \hat{t}} + \hat{\nabla} \cdot \bar{\mathbf{j}}_{\rho}^{\text{C}} = 0, \quad \bar{\mathbf{j}}_{\rho}^{\text{C}} = -\frac{\eta}{n_{\text{D}}/2 + \chi} \left( \hat{\nabla} \bar{\rho}^{\text{C}} + \hat{\nabla} \bar{\phi}^{\text{C}} \right), \quad (\text{S.6-C})$$

$$-\eta^2 \hat{\nabla}^2 \bar{\phi}^{\text{C}} = \bar{\rho}^{\text{C}}. \quad (\text{S.7-C})$$

Due to linearity, the governing equations of the voltage problem are also of the same form

$$\frac{\partial \bar{\rho}^{\text{V}}}{\partial \hat{t}} + \hat{\nabla} \cdot \bar{\mathbf{j}}_{\rho}^{\text{V}} = 0, \quad \bar{\mathbf{j}}_{\rho}^{\text{V}} = -\frac{\eta}{n_{\text{D}}/2 + \chi} \left( \hat{\nabla} \bar{\rho}^{\text{V}} + \hat{\nabla} \bar{\phi}^{\text{V}} \right), \quad (\text{S.6-V})$$

$$-\eta^2 \hat{\nabla}^2 \bar{\phi}^V = \bar{\rho}^V . \quad (\text{S.7-V})$$

Initial conditions for the two subproblems are  $\rho^C(\hat{\mathbf{x}}, \hat{t} = 0) = \rho^V(\hat{\mathbf{x}}, \hat{t} = 0) = 0$ . For the boundary condition at the membrane surface  $\hat{z} = 0$ , Eqs. (S.9) and (S.10) can be written as

$$\bar{\mathbf{j}}_\rho^C \cdot \mathbf{e}_z = \frac{\eta \bar{I}}{n_D/2 + \chi} \frac{\delta(\hat{r})}{2\pi \hat{r}} , \quad (\text{S.9-C})$$

$$\bar{\phi}^C = \eta \chi \frac{\partial \bar{\phi}^C}{\partial \hat{z}} , \quad (\text{S.10-C})$$

$$\bar{\mathbf{j}}_\rho^V \cdot \mathbf{e}_z = 0 , \quad (\text{S.9-V})$$

$$\bar{\phi}^V = \eta \chi \frac{\partial \bar{\phi}^V}{\partial \hat{z}} , \quad (\text{S.10-V})$$

where we assign the transmembrane ionic current to the current-driven problem and the no-flux boundary condition to the voltage-driven problem. Finally, the boundary conditions (S.12)-(S.14) at the electrode surface  $\hat{z} = 1$  are decomposed as

$$\bar{\phi}^C = 0 , \quad (\text{S.12-C})$$

$$\bar{\mathbf{j}}_\rho^C \cdot \mathbf{e}_z = 0 \quad (\text{Blocking}) , \quad (\text{S.13-C})$$

$$\bar{\rho}^C = 0 \quad (\text{Faradaic}) , \quad (\text{S.14-C})$$

$$\bar{\phi}^V = \bar{V} , \quad (\text{S.12-V})$$

$$\bar{\mathbf{j}}_\rho^V \cdot \mathbf{e}_z = 0 \quad (\text{Blocking}) , \quad (\text{S.13-V})$$

$$\bar{\rho}^V = 0 \quad (\text{Faradaic}) . \quad (\text{S.14-V})$$

Equations (S.6-C)-(S.14-C) and Eqs. (S.12-V)-(S.14-V) completely specify the decomposition of the full problem. Since the voltage-driven problem has been analyzed in detail in Ref. [4], we focus on the current-driven problem and, for the sake of brevity, omit superscripts C henceforth.

### III. Boundary layer theory

This section applies matched asymptotic expansions to obtain leading-order solutions of the current-driven problem, resulting in the boundary layer theory. We first construct the *outer* (bulk) solution, then resolve the *inner* (diffuse layer) solutions adjacent to the membrane and the electrode, and finally match the two to obtain a single approximation that is valid throughout the domain.

#### 1. Bulk electrolyte

Combining the charge balance (S.6-C) with the Poisson equation (S.7-C) gives

$$(n_D/2 + \chi) \eta \frac{\partial \bar{\rho}}{\partial \hat{t}} - \eta^2 \hat{\nabla}^2 \bar{\rho} + \bar{\rho} = 0 . \quad (\text{S.16})$$

Because the Debye length is tiny compared with the electrode-membrane spacing ( $\eta = \lambda_D/L \ll 1$ ), we write asymptotic expansions of the bulk fields as

$$\bar{\rho} = \bar{\rho}^b(\hat{\mathbf{x}}, \hat{t}; \eta) \sim \sum_{n=0}^{\infty} \eta^n \bar{\rho}_n^b(\hat{\mathbf{x}}, \hat{t}) , \quad (\text{S.17})$$

$$\bar{\phi} = \bar{\phi}^b(\hat{\mathbf{x}}, \hat{t}; \eta) \sim \sum_{n=0}^{\infty} \eta^n \bar{\phi}_n^b(\hat{\mathbf{x}}, \hat{t}) , \quad (\text{S.18})$$

where the superscript ‘b’ denotes *bulk*. These expansions are valid in the bulk electrolyte region where the diffusive term  $\hat{\nabla}^2 \bar{\rho}$  is bounded. Substituting Eq. (S.17) into Eq. (S.16) and collecting like powers of  $\eta$  yields

$$\bar{\rho}_0^b + \eta \left[ (n_D/2 + \chi) \frac{\partial \bar{\rho}_0^b}{\partial \hat{t}} + \bar{\rho}_1^b \right] + \sum_{n=2}^{\infty} \eta^n \left[ (n_D/2 + \chi) \frac{\partial \bar{\rho}_{n-1}^b}{\partial \hat{t}} - \hat{\nabla}^2 \bar{\rho}_{n-2}^b + \bar{\rho}_n^b \right] = 0 . \quad (\text{S.19})$$

It is straightforward to show that

$$\bar{\rho}_n^b(\hat{\mathbf{x}}, \hat{t}) = 0 \quad (n = 0, 1, 2, \dots) . \quad (\text{S.20})$$

Thus, to all orders, the bulk electrolyte remains electroneutral. This is a consequence of the sink in the charge balance (S.16) being the dominant term—charge separations in the macroscopic length scale  $L$ , if any, diminish quickly due to the large electrostatic driving force. Any net charge injected by the membrane current is confined to narrow diffuse charge layers at the interfaces.

With  $\bar{\rho}_n^b = 0$ , the bulk electric potential is harmonic at all orders and satisfies Laplace’s equation

$$\hat{\nabla}^2 \bar{\phi}_n^b = 0 \quad (n = 0, 1, 2, \dots) , \quad (\text{S.21})$$

subject to boundary conditions supplied by the inner regions, as shown below.

## 2. Diffuse layer at the membrane surface

Near the membrane ( $\hat{z} = 0$ ) we introduce the stretched coordinate  $\bar{z} = \hat{z}/\eta = z/\lambda_D$ . Writing the governing Eqs. (S.16) and (S.7-C) in  $\bar{z}$ , we obtain

$$(n_D/2 + \chi) \eta \frac{\partial \bar{\rho}}{\partial \hat{t}} - \frac{\partial^2 \bar{\rho}}{\partial \bar{z}^2} - \eta^2 \frac{1}{\hat{r}} \frac{\partial}{\partial \hat{r}} \left( \hat{r} \frac{\partial \bar{\rho}}{\partial \hat{r}} \right) + \bar{\rho} = 0 , \quad (\text{S.22})$$

$$-\frac{\partial^2 \bar{\phi}}{\partial \bar{z}^2} - \eta^2 \frac{1}{\hat{r}} \frac{\partial}{\partial \hat{r}} \left( \hat{r} \frac{\partial \bar{\phi}}{\partial \hat{r}} \right) = \bar{\rho} , \quad (\text{S.23})$$

The boundary conditions (S.9-C) and (S.10-C) at the membrane surface  $\bar{z} = 0$  are also rescaled as

$$\frac{\partial}{\partial \bar{z}} (\bar{\rho} + \bar{\phi}) = -\eta \bar{I} \frac{\delta(\hat{r})}{2\pi \hat{r}} , \quad (\text{S.24})$$

$$\bar{\phi} = \chi \frac{\partial \bar{\phi}}{\partial \bar{z}} . \quad (\text{S.25})$$

Asymptotic expansions of  $\bar{\rho}$  and  $\bar{\phi}$  in the membrane-side (m) diffuse layer (inner region) are

$$\bar{\rho} = \bar{\rho}^m(\hat{r}, \bar{z}, \hat{t}; \eta) \sim \sum_{n=0}^{\infty} \eta^n \bar{\rho}_n^m(\hat{r}, \bar{z}, \hat{t}) , \quad (\text{S.26})$$

$$\bar{\phi} = \bar{\phi}^m(\hat{r}, \bar{z}, \hat{t}; \eta) \sim \sum_{n=0}^{\infty} \eta^n \bar{\phi}_n^m(\hat{r}, \bar{z}, \hat{t}) . \quad (\text{S.27})$$

Substituting these expansions into Eqs. (S.22)-(S.25), we obtain leading-order governing equations as

$$-\frac{\partial^2 \bar{\rho}_0^m}{\partial \bar{z}^2} + \bar{\rho}_0^m = 0 , \quad (\text{S.28})$$

$$-\frac{\partial^2 \bar{\phi}_0^m}{\partial \bar{z}^2} = \bar{\rho}_0^m , \quad (\text{S.29})$$

together with the no-flux and Robin boundary conditions

$$\frac{\partial}{\partial \bar{z}} (\bar{\rho}_0^m + \bar{\phi}_0^m) \Big|_{\bar{z}=0} = 0 , \quad (\text{S.30})$$

$$\phi_0^{\text{m}}|_{\bar{z}=0} = \chi \frac{\partial \phi_0^{\text{m}}}{\partial \bar{z}} \Big|_{\bar{z}=0} . \quad (\text{S.31})$$

The leading order solutions are

$$\bar{\rho}_0^{\text{m}}(\hat{r}, \bar{z}, \hat{t}) = \bar{\sigma}_0^{\text{m}}(\hat{r}, \hat{t}) e^{-\bar{z}} , \quad (\text{S.32})$$

$$\bar{\phi}_0^{\text{m}}(\hat{r}, \bar{z}, \hat{t}) = \bar{\sigma}_0^{\text{m}}(\hat{r}, \hat{t}) (1 - e^{-\bar{z}} + \chi) , \quad (\text{S.33})$$

where  $\bar{\sigma}_0^{\text{m}}(\hat{r}, \hat{t})$  is the dimensionless areal charge density at the membrane surface, corresponding to the dimensional  $\sigma^{\text{m}}(r, t)$  in the main text. Because of the decaying exponential in Eq. (S.32), the inner solution matches the outer solution, i.e.  $\bar{\rho}_0^{\text{m}} \rightarrow \bar{\rho}_0^{\text{b}} = 0$  as  $\bar{z} \rightarrow \infty$ . The leading order solutions (S.20), (S.32), and (S.33) together show that the bulk electrolyte stays charge neutral at all times but admits nonzero electric fields from Eq. (S.21). All the “extra” charges reside in the boundary layers near the membrane surface and the electrode surface (see below).

Equations (S.32) and (S.33) indicate that the axial variation at each radial location is always exponential. To focus on the radial and temporal variation, we integrate the charge balance (S.6-C) across the diffuse layer

$$\int_0^{\eta^{1/2}} \left[ \frac{\partial \bar{\rho}}{\partial \hat{t}} - \frac{\eta}{n_{\text{D}}/2 + \chi} \frac{1}{\hat{r}} \frac{\partial}{\partial \hat{r}} \left( \hat{r} \frac{\partial}{\partial \hat{r}} (\bar{\rho} + \bar{\phi}) \right) \right] d\hat{z} - \frac{\eta}{n_{\text{D}}/2 + \chi} \int_0^{\eta^{1/2}} \frac{\partial^2}{\partial \hat{z}^2} (\bar{\rho} + \bar{\phi}) d\hat{z} = 0 . \quad (\text{S.34})$$

Note that the inner solutions are valid throughout the integration interval and that the outer solutions are valid at  $\hat{z} = \eta^{1/2}$  ( $\gg \eta$ ) since  $\bar{\nabla}^2 \bar{\rho}$  is bounded there. The first integral in Eq. (S.34) is computed by substituting the inner solutions and by changing the variable from  $\hat{z}$  to  $\bar{z} = \hat{z}/\eta$  as

$$\eta \frac{\partial \bar{\sigma}_0^{\text{m}}}{\partial \hat{t}} (1 - e^{-\eta^{-1/2}}) - \eta^{3/2} \frac{1 + \chi}{n_{\text{D}}/2 + \chi} \frac{1}{\hat{r}} \frac{\partial}{\partial \hat{r}} \left( \hat{r} \frac{\partial \bar{\sigma}_0^{\text{m}}}{\partial \hat{r}} \right) + \mathcal{O}(\eta^{3/2}) . \quad (\text{S.35})$$

The second integral in Eq. (S.34) is easily integrated to yield two boundary terms, one at the membrane surface and the other at  $\hat{z} = \eta^{1/2}$ . The former can be expressed using the boundary condition (S.9-C),

$$\frac{\partial}{\partial \hat{z}} (\bar{\rho} + \bar{\phi}) \Big|_{\hat{z}=0} = -\bar{I} \frac{\delta(\hat{r})}{2\pi \hat{r}} . \quad (\text{S.36})$$

The boundary term at  $\hat{z} = \eta^{1/2}$  can be expressed using the leading order outer solutions  $\bar{\rho}_0^{\text{b}} = 0$  and  $\bar{\phi}_0^{\text{b}}$ . Thus, Eq. (S.34) becomes

$$\eta \frac{\partial \bar{\sigma}_0^{\text{m}}}{\partial \hat{t}} (1 - e^{-\eta^{-1/2}}) - \frac{\eta}{n_{\text{D}}/2 + \chi} \left( \frac{\partial \bar{\phi}_0^{\text{b}}}{\partial \hat{z}} \Big|_{\hat{z}=\eta^{1/2}} + \bar{I} \frac{\delta(\hat{r})}{2\pi \hat{r}} \right) = \mathcal{O}(\eta^{3/2}) . \quad (\text{S.37})$$

From the leading order contributions as  $\eta \rightarrow 0$ , we obtain

$$\frac{\partial \bar{\sigma}_0^{\text{m}}}{\partial \hat{t}} = \frac{1}{n_{\text{D}}/2 + \chi} \left( \frac{\partial \bar{\phi}_0^{\text{b}}}{\partial \hat{z}} \Big|_{\hat{z}=0} + \bar{I} \frac{\delta(\hat{r})}{2\pi \hat{r}} \right) , \quad (\text{S.38})$$

which indicates that both the transmembrane current and charge flux from the bulk contribute to the charging rate at the membrane surface. By matching the inner and outer electric potentials, i.e.  $\lim_{\bar{z} \rightarrow \infty} \bar{\phi}^{\text{m}} = \lim_{\hat{z} \rightarrow 0} \bar{\phi}^{\text{b}}$ , the membrane-side areal charge density is related to the bulk electric potential as

$$\bar{\sigma}_0^{\text{m}} (1 + \chi) = \bar{\phi}_0^{\text{b}}|_{\hat{z}=0} . \quad (\text{S.39})$$

Substituting Eq. (S.39) to Eq. (S.38), we obtain

$$\frac{\partial \bar{\phi}_0^{\text{b}}}{\partial \hat{t}} \Big|_{\hat{z}=0} = \frac{1 + \chi}{n_{\text{D}}/2 + \chi} \left( \frac{\partial \bar{\phi}_0^{\text{b}}}{\partial \hat{z}} \Big|_{\hat{z}=0} + \bar{I} \frac{\delta(\hat{r})}{2\pi \hat{r}} \right) , \quad (\text{S.40})$$

which may be rewritten using  $\hat{v}$  as

$$\left. \frac{\partial \bar{\phi}_0^b}{\partial \hat{t}} \right|_{\hat{z}=0} = \hat{v} \left( \left. \frac{\partial \bar{\phi}_0^b}{\partial \hat{z}} \right|_{\hat{z}=0} + \bar{I} \frac{\delta(\hat{r})}{2\pi\hat{r}} \right). \quad (\text{S.41})$$

This serves as one of the two time-dependent boundary condition when solving the Laplace equation (S.21) for the leading order bulk electric potential  $\bar{\phi}_0^b$ . Equation (S.41) can be redimensionalized through the transformations listed in Table S1 to obtain the form presented in Sec. IIIC of the main text. The second boundary condition is derived in the next section.

### 3. Diffuse layer at the electrode surface

For idealized Faradaic electrodes ( $n_D = 2$ ), diffuse charge layers are absent, so no singular perturbation analysis is required at the electrode interface. In what follows, we therefore focus on the case of a blocking electrode. On the electrolyte side near the electrode surface ( $\hat{z} = 1$ ), it is convenient to introduce the stretched coordinate  $\bar{z}' = (1 - \hat{z})/\eta = (L - z)/\lambda_D$ . To that end, the asymptotic expansions in the inner region are

$$\bar{\rho} = \bar{\rho}^e(\hat{r}, \bar{z}', \hat{t}; \eta) \sim \sum_{n=0}^{\infty} \eta^n \bar{\rho}_n^e(\hat{r}, \bar{z}', \hat{t}), \quad (\text{S.42})$$

$$\bar{\phi} = \bar{\phi}^e(\hat{r}, \bar{z}', \hat{t}; \eta) \sim \sum_{n=0}^{\infty} \eta^n \bar{\phi}_n^e(\hat{r}, \bar{z}', \hat{t}). \quad (\text{S.43})$$

Proceeding as in the case of the membrane-side diffuse layer, the leading order governing equations and boundary conditions are given by

$$-\frac{\partial^2 \bar{\rho}_0^e}{\partial \bar{z}'^2} + \bar{\rho}_0^e = 0, \quad (\text{S.44})$$

$$-\frac{\partial^2 \bar{\phi}_0^e}{\partial \bar{z}'^2} = \bar{\rho}_0^e, \quad (\text{S.45})$$

$$\left. \frac{\partial}{\partial \bar{z}'} (\bar{\rho}_0^e + \bar{\phi}_0^e) \right|_{\bar{z}'=0} = 0, \quad (\text{S.46})$$

$$\bar{\phi}_0^e|_{\bar{z}'=0} = 0. \quad (\text{S.47})$$

The inner solutions at the electrode surface are

$$\bar{\rho}_0^e(\hat{r}, \bar{z}', \hat{t}) = \bar{\sigma}_0^e(\hat{r}, \hat{t}) e^{-\bar{z}'}, \quad (\text{S.48})$$

$$\bar{\phi}_0^e(\hat{r}, \bar{z}', \hat{t}) = \bar{\sigma}_0^e(\hat{r}, \hat{t}) (1 - e^{-\bar{z}'}), \quad (\text{S.49})$$

where  $\bar{\sigma}_0^e(\hat{r}, \hat{t})$  is the dimensionless areal charge density at the electrode surface. Analogous to the membrane-side analysis, the evolution of  $\bar{\sigma}_0^e(\hat{r}, \hat{t})$  is obtained by integrating the charge balance Eq. (S.6-C) along the axial direction  $\hat{z}$  from  $1 - \eta^{1/2}$  to 1. At leading order,

$$\frac{\partial \bar{\sigma}_0^e}{\partial \hat{t}} = -\frac{1}{2 + \chi} \left. \frac{\partial \bar{\phi}_0^b}{\partial \hat{z}} \right|_{\hat{z}=1}, \quad (\text{S.50})$$

indicating that the areal charge density at the electrode surface changes due to the charge flux from the bulk. The matching condition, i.e.  $\lim_{\bar{z}' \rightarrow \infty} \bar{\phi}^e = \lim_{\hat{z} \rightarrow 1} \bar{\phi}^b$ , then yields

$$\bar{\sigma}_0^e = \bar{\phi}_0^b|_{\hat{z}=1}. \quad (\text{S.51})$$

Substituting this into Eq. (S.50) and using  $\hat{u} = 1/(2 + \chi)$  for blocking electrodes yields the second time-dependent boundary condition for the Laplace equation (S.21) as

$$\left. \frac{\partial \bar{\phi}_0^b}{\partial \hat{t}} \right|_{\hat{z}=1} = -\hat{u} \left. \frac{\partial \bar{\phi}_0^b}{\partial \hat{z}} \right|_{\hat{z}=1}, \quad (\text{S.52})$$

which is expressed in its dimensional form at the end of Sec. IIIC in the main text. Although the boundary condition (S.41) remains the same regardless of the type of electrode, the condition (S.52) changes to Eq. (S.14-C) for idealized Faradaic electrodes. Although we now proceed with the case of blocking electrodes, the case of Faradaic electrodes will be discussed in Sec. VI.

#### 4. Leading-order uniform solution

The solution strategy is now clear:

1. Solve Laplace's equation (S.21) for  $\bar{\phi}_0^b$  with boundary conditions (S.41) and (S.52) (blocking electrodes) or (S.41) and (S.14-C) (perfect Faradaic electrodes).
2. Recover the areal charge densities from Eq. (S.39) for the membrane-side diffuse layer and Eq. (S.51) for the electrode-side diffuse layer for the case of blocking electrodes. The inner solutions are fully determined by Eqs. (S.32) and (S.33) at the membrane surface and by Eqs. (S.48) and (S.49) at the blocking electrode surface; see Sec. VI for the Faradaic case.
3. Assemble the uniformly valid leading-order fields by adding the inner and outer contributions and subtracting their overlap, for instance:

$$\bar{\phi}_0^{\text{uniform}}(\hat{r}, \hat{z}, \hat{t}) = \bar{\phi}_0^m(\hat{r}, \hat{z}/\eta, \hat{t}) + \bar{\phi}_0^b(\hat{r}, \hat{z}, \hat{t}) + \bar{\phi}_0^e(\hat{r}, (1 - \hat{z})/\eta, \hat{t}) - \bar{\phi}_0^b(\hat{r}, 0, \hat{t}) - \bar{\phi}_0^b(\hat{r}, 1, \hat{t}), \quad (\text{S.53})$$

when considering potential in the case of blocking electrodes. This yields the following charge density and electric potential fields:

$$\bar{\rho}_0^{\text{uniform}}(\hat{r}, \hat{z}, \hat{t}) = \begin{cases} \bar{\sigma}_0^m(\hat{r}, \hat{t})e^{-\hat{z}/\eta} + \bar{\sigma}_0^e(\hat{r}, \hat{t})e^{-(1-\hat{z})/\eta} & (\text{Blocking}) \\ \bar{\sigma}_0^m(\hat{r}, \hat{t})e^{-\hat{z}/\eta} & (\text{Faradaic}) \end{cases}, \quad (\text{S.54})$$

$$\bar{\phi}_0^{\text{uniform}}(\hat{r}, \hat{z}, \hat{t}) = \begin{cases} \bar{\phi}_0^b(\hat{r}, \hat{t}) - \bar{\sigma}_0^m(\hat{r}, \hat{t})e^{-\hat{z}/\eta} - \bar{\sigma}_0^e(\hat{r}, \hat{t})e^{-(1-\hat{z})/\eta} & (\text{Blocking}) \\ \bar{\phi}_0^b(\hat{r}, \hat{t}) - \bar{\sigma}_0^m(\hat{r}, \hat{t})e^{-\hat{z}/\eta} & (\text{Faradaic}) \end{cases}. \quad (\text{S.55})$$

From Eqs. (S.33) and (S.39), the dimensionless transmembrane potential is given by

$$\bar{V}^M = 2\chi\bar{\sigma}_0^m = \frac{2\chi}{1+\chi} \bar{\phi}_0^b|_{\hat{z}=0}, \quad (\text{S.56})$$

in terms of the bulk potential. The factor of  $\chi/(1+\chi) = C_M^{\text{eq}}/C_M$  is the ratio of the total capacitance of the membrane and its adjacent diffuse charge layers to the capacitance of the membrane alone, which is close to 1 for typical physiological settings.

## IV. Early time solution: Point-charge approximation

At early times  $t \ll \tau_D$ , there is limited diffuse charge reorganization, and the pumped charge stays localized near the transporter patch. This motivates the *point-charge approximation* introduced in Ref. [5], in which the transported charges are represented by a point positive charge of magnitude  $Q \equiv It$  at the transporter outlet and a point negative charge of magnitude  $-Q$  at the inlet. The electrolyte solutions are treated as perfect dielectrics with zero free charge everywhere except at the location of the point charges. The resulting electric potential, denoted  $\phi^{\text{pc}}$ , is obtained by solving Poisson's equation with the point charges as sources.

In the unbounded system case considered in Ref. [5], this problem admits an exact solution using Hankel transforms. Therefore, we first attempted the same approach on the electrode-bounded system considered in this work. Unfortunately, the grounding boundary conditions at the electrode surfaces led to more complicated expressions in Hankel space that could not be inverted in closed form. Efforts to extract simple asymptotic forms to match the numerical simulations were also unsuccessful. We next tried an eigenfunction expansion in the bounded  $z$  direction (à la Sturm-Liouville), but this also proved intractable. The radial coefficients in the expansion involved modified Bessel functions of the second kind, whose divergences near  $r \rightarrow 0$  prevented proper matching to the  $\delta$ -function point sources.



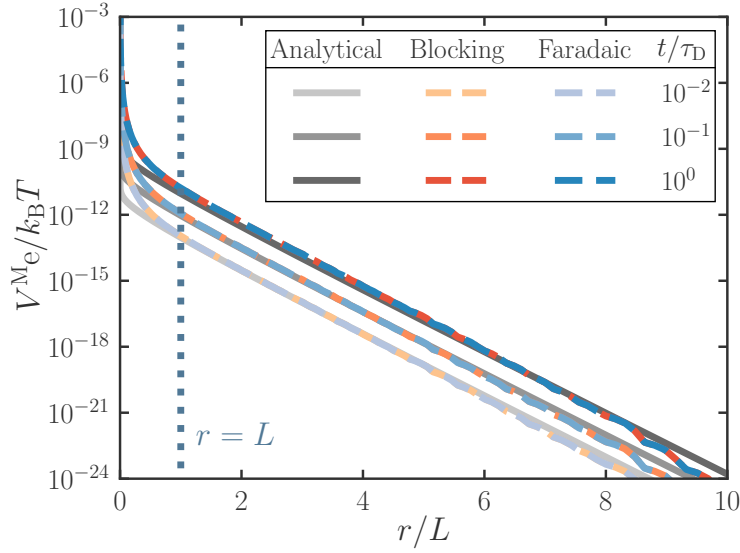

Figure S2: The electrostatics in the far-field. The analytical result of Eq. (S.61) is plotted against the numerical solutions in the case of both blocking and Faradaic electrodes. We see that the solution captures the correct behavior. Simulation parameters as in Fig. 3 of the main text. The disagreement near  $r = 10L$  is caused by machine precision error.

Once specified,  $\phi^{\text{pc}}$  follows simply from superposing the Coulombic contributions of the original and image charges.

For the unbounded system, the image charge representation (illustrated in Fig. S1(a)) leads to a potential that is monopolar with effective charge  $\approx 2Q$  in the near field ( $r' \ll \Gamma\delta^{\text{M}}$ ), where  $r' = \sqrt{r^2 + z^2}$  is the distance from the transporter. At larger distances  $r' \gg \Gamma\delta^{\text{M}}$ , the potential is dipolar with dipole moment  $Q\Gamma\delta^{\text{M}}\mathbf{e}_z$ . On the other hand, for the bounded system, the appropriate set of image charges must enforce the grounding condition ( $\phi = 0$ ) at the two electrodes. This can be accomplished by supplementing the original system by an infinite sequence of reflected “image systems” along  $z$ , as represented in Fig. S1(b). Each image is  $2L + \Gamma\delta^{\text{M}}$  thick along  $z$ , and contains point dipole of moment  $Q\Gamma\delta^{\text{M}}\mathbf{e}_z$  at its center and two grounded electrodes above and below. The potential at any point in the original domain is obtained by superposing the contributions the original dipole and all image dipoles.

We now evaluate the potential  $\phi^{\text{pc}}$  for the bounded system, beginning with the near-field  $r' \ll \Gamma\delta^{\text{M}}$ . From Ref. [5], the point dipole in the original system contributes as a monopole at this short range. However, since  $L \gg \Gamma\delta^{\text{M}}$ , each reflected system contributes a dipolar field in these locations. At leading order, the monopolar contribution will dominate, giving

$$\phi^{\text{pc}}(r, z) \approx \frac{1}{4\pi\epsilon} \frac{2Q}{\sqrt{z^2 + r^2}}. \quad (\text{S.57})$$

By contrast, in the region  $r' \gg \Gamma\delta^{\text{M}}$ , the original system makes a dipolar contribution. The condition  $L \gg \Gamma\delta^{\text{M}}$  guarantees that the reflected images are well separated from the location, so their contributions also enter only as dipolar fields. The electric potential for  $r \gg \Gamma\delta^{\text{M}}$  is then a superposition of an infinite series of dipoles

$$\phi^{\text{pc}}(r, z) = \frac{Q\Gamma\delta^{\text{M}}}{4\pi\epsilon} \sum_{m=-\infty}^{\infty} \frac{(2L + \Gamma\delta^{\text{M}})m + \Gamma\delta^{\text{M}}/2 + z}{(((2L + \Gamma\delta^{\text{M}})m + \Gamma\delta^{\text{M}}/2 + z)^2 + r^2)^{3/2}}. \quad (\text{S.58})$$

For  $r \ll L$ , the  $m = 0$  term dominates, and the potential essentially coincides with that of the original dipole in an unbounded medium. Contributions from  $m \neq 0$  images only become relevant at distances comparable to the electrode separation  $L$ .

For  $r > L$ , it is more convenient to recast the potential in terms of an eigenfunction (spectral) representation (see Appendix A for derivation). Using the case of  $p = 0$  in Eq. (S.166) yields

$$\phi^{\text{pc}}(r, z) = \frac{It\Gamma\delta^{\text{M}}}{2\epsilon(L + \Gamma\delta^{\text{M}}/2)^2} \sum_{n=1}^{\infty} nK_0\left(\frac{n\pi r}{L + \Gamma\delta^{\text{M}}/2}\right) \sin\left(\frac{n\pi(z + \Gamma\delta^{\text{M}}/2)}{L + \Gamma\delta^{\text{M}}/2}\right), \quad (\text{S.59})$$

where  $K_0$  is the zeroth-order modified Bessel function of the second kind. Because  $K_0(x) \sim e^{-x}\sqrt{\pi/2x}$  for large  $x$ , the  $n = 1$  term dominates in the far-field. Thus for  $r \gg L$ ,

$$\phi^{\text{pc}}(r, z) \approx \frac{It\Gamma\delta^{\text{M}}}{2\epsilon L^2} K_0\left(\frac{\pi r}{L + \Gamma\delta^{\text{M}}/2}\right) \sin\left(\frac{\pi(z + \Gamma\delta^{\text{M}}/2)}{L + \Gamma\delta^{\text{M}}/2}\right). \quad (\text{S.60})$$

Evaluating this field on the membrane surface  $z = 0$  and Taylor series expanding the remaining sine term using  $\Gamma\delta^{\text{M}} \ll L$  gives the transmembrane potential

$$V_{\text{pc}}^{\text{M}}(r) \equiv 2\phi^{\text{pc}}(r, 0) = \frac{2\pi It}{\epsilon L} \left(\frac{\chi\lambda_{\text{D}}}{L}\right)^2 K_0\left(\frac{\pi r}{L}\right) \left(1 + \mathcal{O}\left(\frac{\chi\lambda_{\text{D}}}{L}\right)\right), \quad (\text{S.61})$$

where we have substituted  $\Gamma\delta^{\text{M}} = 2\chi\lambda_{\text{D}}$ . Equation (S.61) is quoted in the main text [Eq.(19)] as the early-time, far-field ( $r \gg L$ ) transmembrane potential. Its derivation relies only on the presence of grounded electrodes at  $z \approx \pm L$ , and is therefore valid for both blocking and Faradaic electrodes, as verified in Fig.S2.

## V. Late time solutions: Blocking electrodes

For  $t \gg \tau_{\text{D}}$ , diffuse charges reorganize throughout the system and the point charge approximation is not applicable. For the case of blocking electrodes, the leading-order diffuse charge dynamics are governed by the boundary layer formulation encapsulated in Eqs. (S.21), (S.41), and (S.52). The governing equations for the leading order bulk electric potential are:

$$0 = \frac{1}{\hat{r}} \frac{\partial}{\partial \hat{r}} \left( \hat{r} \frac{\partial \bar{\phi}_0^{\text{b}}}{\partial \hat{r}} \right) + \frac{\partial^2 \bar{\phi}_0^{\text{b}}}{\partial \hat{z}^2}, \quad (\text{S.62})$$

$$\left. \frac{\partial \bar{\phi}_0^{\text{b}}}{\partial \hat{t}} \right|_{\hat{z}=0} = \hat{v} \left( \left. \frac{\partial \bar{\phi}_0^{\text{b}}}{\partial \hat{z}} \right|_{\hat{z}=0} + \bar{I} \frac{\delta(\hat{r})}{2\pi\hat{r}} \right), \quad (\text{S.63})$$

$$\left. \frac{\partial \bar{\phi}_0^{\text{b}}}{\partial \hat{t}} \right|_{\hat{z}=1} = -\hat{u} \left. \frac{\partial \bar{\phi}_0^{\text{b}}}{\partial \hat{z}} \right|_{\hat{z}=1}, \quad (\text{S.64})$$

subjected to the initial condition  $\bar{\phi}_0^{\text{b}}(\hat{r}, \hat{z}, 0) = 0$ . This system of equations can be solved by employing the Hankel transform in  $\hat{r}$ , defined as [7, 8]

$$\hat{\phi}_0^{\text{b}}(\hat{k}, \hat{z}, \hat{t}) = \int_0^\infty d\hat{r} \hat{r} J_0(\hat{k}\hat{r}) \bar{\phi}_0^{\text{b}}(\hat{r}, \hat{z}, \hat{t}). \quad (\text{S.65})$$

Because the Hankel transform is self-reciprocal, applying it once more in  $\hat{k}$  recovers the original real-space function. Applying the transform to Eqs. (S.62)-(S.64) gives

$$0 = -\hat{k}^2 \hat{\phi}_0^{\text{b}} + \frac{\partial^2 \hat{\phi}_0^{\text{b}}}{\partial \hat{z}^2}, \quad (\text{S.66})$$

$$\left. \frac{\partial \hat{\phi}_0^{\text{b}}}{\partial \hat{t}} \right|_{\hat{z}=0} = \hat{v} \left( \left. \frac{\partial \hat{\phi}_0^{\text{b}}}{\partial \hat{z}} \right|_{\hat{z}=0} + \frac{\bar{I}}{2\pi} \right), \quad (\text{S.67})$$

$$\left. \frac{\partial \hat{\phi}_0^{\text{b}}}{\partial \hat{t}} \right|_{\hat{z}=1} = -\hat{u} \left. \frac{\partial \hat{\phi}_0^{\text{b}}}{\partial \hat{z}} \right|_{\hat{z}=1}. \quad (\text{S.68})$$

Equation (S.66) has the general solution

$$\hat{\phi}_0^b(\hat{k}, \hat{z}, \hat{t}) = \hat{\phi}_0^b(\hat{k}, 0, \hat{t}) \frac{\sinh(\hat{k}(1 - \hat{z}))}{\sinh(\hat{k})} + \hat{\phi}_0^b(\hat{k}, 1, \hat{t}) \frac{\sinh(\hat{k}\hat{z})}{\sinh(\hat{k})}, \quad (\text{S.69})$$

where the functions  $\hat{\phi}_0^b(\hat{k}, 0, \hat{z})$  and  $\hat{\phi}_0^b(\hat{k}, 1, \hat{z})$  surfaces are yet to be determined. With the matching conditions (S.39) and (S.51), they are directly related to the transformed areal charge densities,

$$\hat{\sigma}_0^m(\hat{k}, \hat{t}) = \frac{\hat{\phi}_0^b(\hat{k}, 0, \hat{t})}{1 + \chi}, \quad (\text{S.70})$$

$$\hat{\sigma}_0^e(\hat{k}, \hat{t}) = \hat{\phi}_0^b(\hat{k}, 1, \hat{t}). \quad (\text{S.71})$$

Here,  $\hat{\sigma}_0^m(\hat{k}, \hat{t})$  and  $\hat{\sigma}_0^e(\hat{k}, \hat{t})$  are Hankel transforms of  $\bar{\sigma}_0^m(\hat{r}, \hat{t})$  and  $\bar{\sigma}_0^e(\hat{r}, \hat{t})$ , respectively. Accordingly,  $\hat{\phi}_0^b(\hat{k}, 0, \hat{t})$  and  $\hat{\phi}_0^b(\hat{k}, 1, \hat{t})$  can be used to determine the charge density and electric potential in the membrane-side and electrode-side diffuse charge layers via Eqs. (S.32), (S.33), (S.48), and (S.49).

Applying (S.67) and (S.68), we obtain a coupled linear ODE system governing the time evolution of  $\hat{\phi}_0^b(\hat{k}, 0, \hat{t})$  and  $\hat{\phi}_0^b(\hat{k}, 1, \hat{t})$

$$\frac{\partial}{\partial \hat{t}} \begin{bmatrix} \hat{\phi}_0^b(\hat{k}, 0, \hat{t}) \\ \hat{\phi}_0^b(\hat{k}, 1, \hat{t}) \end{bmatrix} = -\frac{\hat{k}}{\tanh(\hat{k})} \begin{bmatrix} \hat{v} & -\hat{v} \operatorname{sech}(\hat{k}) \\ -\hat{u} \operatorname{sech}(\hat{k}) & \hat{u} \end{bmatrix} \begin{bmatrix} \hat{\phi}_0^b(\hat{k}, 0, \hat{t}) \\ \hat{\phi}_0^b(\hat{k}, 1, \hat{t}) \end{bmatrix} + \hat{v} \begin{bmatrix} \bar{I}/2\pi \\ 0 \end{bmatrix}. \quad (\text{S.72})$$

The associated initial conditions are

$$\hat{\phi}_0^b(\hat{k}, 0, 0) = \hat{\phi}_0^b(\hat{k}, 1, 0) = 0. \quad (\text{S.73})$$

The matrix in Eq. (S.72) admits two eigenvalues, whose reciprocals are the governing timescales:

$$\hat{s}_{\pm}(\hat{k}) = \frac{1}{2} \frac{\hat{k}}{\tanh(\hat{k})} \left[ 1 \pm \sqrt{1 - 4\hat{u}\hat{v} \tanh^2(\hat{k})} \right], \quad (\text{S.74})$$

where we use  $\hat{u} + \hat{v} = 1$ . Because  $\chi \gg 1$ , we have  $\hat{u} = 1/(2 + \chi) \ll 1$ , so the factor under the square root

$$\hat{d} \equiv 4\hat{u}\hat{v} \tanh^2(\hat{k}) \ll 1, \quad (\text{S.75})$$

for all  $\hat{k} \geq 0$ . Consequently,  $\hat{s}_{\pm}$  are real and the system response is not oscillatory.

Two limiting cases are particularly informative. In the small wavelength ( $\hat{k} \gg 1$ ) limit,  $\tanh(\hat{k}) \rightarrow 1$  and Eq. (S.74) yields

$$\hat{s}_+ \sim \hat{s}_+^{\infty} = \hat{k}\hat{v}, \quad (\text{S.76a})$$

$$\hat{s}_- \sim \hat{s}_-^{\infty} = \hat{k}\hat{u}. \quad (\text{S.76b})$$

In this limit Eqs. (S.72) decouple and reduce to

$$\frac{\partial \hat{\phi}_0^b(\hat{k}, 0, \hat{t})}{\partial \hat{t}} \approx -\hat{s}_+^{\infty} \hat{\phi}_0^b(\hat{k}, 0, \hat{t}) + \hat{v} \frac{\bar{I}}{2\pi}, \quad (\text{S.77})$$

$$\frac{\partial \hat{\phi}_0^b(\hat{k}, 1, \hat{t})}{\partial \hat{t}} \approx -\hat{s}_-^{\infty} \hat{\phi}_0^b(\hat{k}, 1, \hat{t}), \quad (\text{S.78})$$

which shows that  $\hat{s}_+^{\infty}$  and  $\hat{s}_-^{\infty}$  correspond to timescales governing the dynamics in the near-field region. Furthermore, from the linear dependence  $\hat{s}_{\pm}^{\infty} \propto \hat{k} \gg 1$ , we expect front-like behaviors along the radial direction for  $r \ll L$  during initial dynamics. This shows the roles of  $\hat{u}$  and  $\hat{v}$  as propagation velocities in the radial direction.

In the large wavelength ( $\hat{k} \ll 1$ ) limit, Eq. (S.74) simplifies to

$$\hat{s}_+ \sim \hat{s}_+^0 = 1, \quad (\text{S.79a})$$

$$\hat{s}_- \sim \hat{s}_-^0 = \hat{u}\hat{v}\hat{k}^2. \quad (\text{S.79b})$$

Thus, the characteristic time  $1/\hat{s}_+^0$  equals the capacitive timescale  $\tau_C$  used to nondimensionalize the problem. Thus the capacitive timescale, introduced in Ref. [4], governs the leading-order charging dynamics of the membrane- and electrode-side diffuse layers in the far-field  $r \gg L$ . The smaller eigenvalue  $\hat{s}_-^0 \propto \hat{k}^2$  captures a slow, diffusive spreading of the charges at long times, with effective diffusivity  $D_{\text{eff}} = uv\tau_C = ((1+\chi)/(2+\chi))(L^2/\tau_C)$ .

**Exact transform-space solution.** Solving Eq. (S.72) subject to the initial condition (S.73) gives

$$\hat{\phi}_0^b(\hat{k}, 0, \hat{t}) = \frac{\bar{I}}{2\pi \hat{k} \tanh(\hat{k})} \left[ 1 - e^{-\hat{s}_- \hat{t}} + \frac{1}{2} \left( 1 - \frac{1 - \hat{d}/2\hat{u}}{\sqrt{1 - \hat{d}}} \right) (e^{-\hat{s}_- \hat{t}} - e^{-\hat{s}_+ \hat{t}}) \right], \quad (\text{S.80})$$

$$\hat{\phi}_0^b(\hat{k}, 1, \hat{t}) = \frac{\bar{I}}{2\pi \hat{k} \sinh(\hat{k})} \left[ 1 - e^{-\hat{s}_- \hat{t}} - \frac{1}{2} \left( \frac{1}{\sqrt{1 - \hat{d}}} - 1 \right) (e^{-\hat{s}_- \hat{t}} - e^{-\hat{s}_+ \hat{t}}) \right], \quad (\text{S.81})$$

where  $\hat{d}(\hat{k}) = 4\hat{u}\hat{v} \tanh^2(\hat{k})$ .

## 1. Near-field ( $r < L$ ) solution

To analyze the near-field solution, we consider the small-wavelength limit of  $\hat{k} \gg 1$ . In this limit, we have  $\tanh(\hat{k}) \rightarrow 1$ . Accordingly,  $\hat{d} \rightarrow 4\hat{u}\hat{v}$  and  $\sqrt{1 - \hat{d}} \rightarrow \hat{v} - \hat{u}$ , and we may approximate Eqs. (S.80) and (S.81) as

$$\hat{\phi}_0^b(\hat{k}, 0, \hat{t}) = \frac{\bar{I}}{2\pi \hat{k}} (1 - e^{-\hat{v}\hat{k}\hat{t}}), \quad (\text{S.82})$$

$$\hat{\phi}_0^b(\hat{k}, 1, \hat{t}) = \frac{\bar{I}}{2\pi \hat{k}} 2e^{-\hat{k}} \left( 1 - \frac{1}{1 - \frac{\hat{u}}{\hat{v}}} e^{-\hat{u}\hat{k}\hat{t}} + \frac{1}{\frac{\hat{v}}{\hat{u}} - 1} e^{-\hat{v}\hat{k}\hat{t}} \right). \quad (\text{S.83})$$

This may be exactly inverted to real space as

$$\bar{\phi}_0^b(\hat{r}, 0, \hat{t}) = \frac{\bar{I}}{2\pi} \left( \frac{1}{\hat{r}} - \frac{1}{\sqrt{\hat{r}^2 + (\hat{v}\hat{t})^2}} \right), \quad (\text{S.84})$$

$$\bar{\phi}_0^b(\hat{r}, 1, \hat{t}) = \frac{\bar{I}}{\pi} \left( \frac{1}{\sqrt{\hat{r}^2 + 1}} - \frac{1}{1 - \frac{\hat{u}}{\hat{v}}} \frac{1}{\sqrt{\hat{r}^2 + (1 + \hat{u}\hat{t})^2}} + \frac{1}{\frac{\hat{v}}{\hat{u}} - 1} \frac{1}{\sqrt{\hat{r}^2 + (1 + \hat{v}\hat{t})^2}} \right), \quad (\text{S.85})$$

in the limit of  $\hat{r} \ll 1$ . The solution for  $\bar{\phi}_0^b(\hat{r}, 0, \hat{t})$  exactly recovers the result of Ref. [5] for a membrane in an unbounded domain. Meanwhile, the potential distribution at the electrode shows only a weak dependence on  $\hat{r}$ , as each term in the radical is of the form  $(\hat{r}^2 + 1 + \dots)$ , where the remainder is positive and we are necessarily assuming  $\hat{r} \ll 1$  in the near-field. Therefore, we can approximate  $\bar{\phi}_0^b(\hat{r}, 1, \hat{t})$  in the near-field by its constant value at  $\hat{r} = 0$  given by

$$\bar{\phi}_0^b(0, 1, \hat{t}) = \frac{\bar{I}}{\pi} \frac{1}{\frac{1}{\hat{u}} - \frac{1}{\hat{v}}} \left( \frac{\hat{t}}{1 + \hat{u}\hat{t}} - \frac{\hat{t}}{1 + \hat{v}\hat{t}} \right) = \frac{\bar{I}}{\pi} \frac{\hat{u}\hat{v}\hat{t}^2}{1 + \hat{t} + \hat{u}\hat{v}\hat{t}^2}, \quad (\text{S.86})$$

where we use the identity  $\hat{u} + \hat{v} = 1$ .

Substituting Eqs. (S.84) and (S.85) into Eqs. (S.39) and (S.51), we find the areal charge densities and transmembrane potential to be

$$\bar{\sigma}_0^m(\hat{t}, \hat{r}) = \frac{\bar{I}}{2\pi(1+\chi)} \left( \frac{1}{\hat{r}} - \frac{1}{\sqrt{\hat{r}^2 + (\hat{v}\hat{t})^2}} \right), \quad (\text{S.87})$$

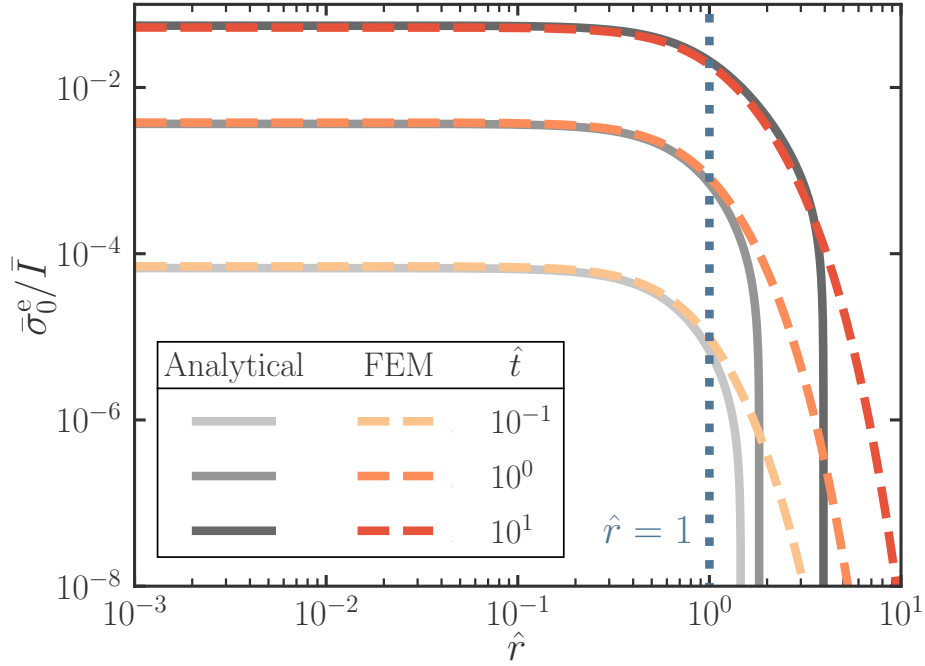

Figure S3: The areal charge density at the electrode. Solid lines are the analytical solution obtained in the small wavelength limit (Eq. (S.88)) and dashed lines are the numerical solution. The analytical solutions are accurate in the near-field ( $\hat{r} < 1$ ).

$$\bar{\sigma}_0^e(\hat{t}, \hat{r}) = \frac{\bar{I}}{\pi} \left( \frac{1}{\sqrt{\hat{r}^2 + 1}} - \frac{\chi + 1}{\chi} \frac{1}{\sqrt{\hat{r}^2 + (1 + \hat{u}\hat{t})^2}} + \frac{1}{\chi} \frac{1}{\sqrt{\hat{r}^2 + (1 + \hat{v}\hat{t})^2}} \right), \quad (\text{S.88})$$

$$\bar{V}^M(\hat{t}, \hat{r}) = \frac{\bar{I}\chi}{\pi(1 + \chi)} \left( \frac{1}{\hat{r}} - \frac{1}{\sqrt{\hat{r}^2 + (\hat{v}\hat{t})^2}} \right), \quad (\text{S.89})$$

in the near field. Redimensionalizing Eq. (S.89) by using Table S1 recovers the expression presented in Sec. IVA of the main text. The analytical solution for the transmembrane potential is compared with the numerical results in the main text. Figure S3 shows good agreement between Eq. (S.88) and numerical results for  $\hat{r} < 1$  near the electrode.

Equations (S.88)-(S.89) suggest that the near-field profiles approach the steady-state monopolar solution of Ref. [5] as  $\hat{t} \rightarrow \infty$ . However, these expressions are only valid until the crossover to the diffusive regime occurs, following which the profiles grow logarithmically with time, eventually diverging. The reason behind this apparent discrepancy is explained in more detail below at the end of Sec. V.3.

## 2. Far-field, capacitive regime ( $r > L$ , $\tau_D < t < r/v$ )

In the dimensionless formulation, the capacitive regime corresponds to  $\hat{t} < \hat{r}$ . Although the existence of this regime was motivated based on simulations in the main text, it can also be inferred from Eqs. (S.80) and (S.81), which govern the dynamics of  $\hat{\phi}_0^b(\hat{k}, 0, \hat{t})$  and  $\hat{\phi}_0^b(\hat{k}, 1, \hat{t})$ . To see this, consider the Laplace transform, which is defined for a time-dependent function as  $\mathcal{L}[f](\hat{s}) = \int_0^\infty f(t)e^{-\hat{s}t} d\hat{t}$ . Applying the Laplace transform to Eqs. (S.80) and (S.81), we obtain

$$\mathcal{L}[\hat{\phi}_0^b](\hat{k}, 0, \hat{s}) = \frac{\bar{I}}{2\pi\hat{s}} \frac{\hat{v}\hat{s} \sinh(\hat{k}) + \hat{u}\hat{v}\hat{k} \cosh(\hat{k})}{\left(\hat{u}\hat{v}\hat{k}^2 + \hat{s}^2\right) \sinh(\hat{k}) + \hat{k}\hat{s} \cosh(\hat{k})}, \quad (\text{S.90})$$

$$\mathcal{L}[\hat{\phi}_0^b](\hat{k}, 1, \hat{s}) = \frac{\bar{I}}{2\pi\hat{s}} \frac{\hat{u}\hat{v}\hat{k}}{(\hat{u}\hat{v}\hat{k}^2 + \hat{s}^2) \sinh(\hat{k}) + \hat{k}\hat{s} \cosh(\hat{k})}. \quad (\text{S.91})$$

Now consider the asymptotic limit  $\hat{t} \ll \hat{r}$ , which corresponds to  $\hat{s} \gg \hat{k}$  in the transformed space. In this limit, we may neglect the term  $\hat{k}^2 \sinh(\hat{k})$  in the denominator of Eqs. (S.90) and (S.91), but keep the other two terms. We keep the other two terms to retain the controlling pole of the transformed solution. This yields the simpler expressions,

$$\mathcal{L}[\hat{\phi}_0^b](\hat{k}, 0, \hat{s}) = \frac{\bar{I}}{2\pi\hat{s}} \hat{v}^2 \frac{1}{\hat{s} + \hat{k}/\tanh(\hat{k})} + \frac{\bar{I}\hat{u}\hat{v}}{2\pi\hat{s}^2}, \quad (\text{S.92})$$

$$\mathcal{L}[\hat{\phi}_0^b](\hat{k}, 1, \hat{s}) = \frac{\bar{I}}{2\pi\hat{s}^2} \hat{u}\hat{v} \frac{\hat{k}/\sinh(\hat{k})}{\hat{s} + \hat{k}/\tanh(\hat{k})}. \quad (\text{S.93})$$

The last term in Eq. (S.92) is singular at  $\hat{r} = 0$ , which when inverted to real space corresponds to the near-field variation not captured by the first term. Principally, the singularity arises from neglecting the second pole in Eq. (S.90) which become relevant for  $\hat{t} \gtrsim \hat{r}$ . However, it is valid to neglect this term for  $\hat{t} \ll \hat{r}$  and  $\hat{r} \gg 1$ .

In the far field ( $\hat{r} \gg 1$  or  $\hat{k} \ll 1$ ), where  $\hat{k}/\tanh(\hat{k}) \rightarrow 1$ , we obtain Laurent expansions of the above expressions about  $\hat{s} = -1$ . Note that

$$\frac{1}{\hat{s} + \hat{k}/\tanh(\hat{k})} = \sum_{n=0}^{\infty} \frac{1}{(\hat{s} + 1)^{n+1}} \left(1 - \frac{\hat{k}}{\tanh(\hat{k})}\right)^n. \quad (\text{S.94})$$

Using this series, Eqs. (S.92) and (S.93) are written as

$$\mathcal{L}[\hat{\phi}_0^b](\hat{k}, 0, \hat{s}) \approx \frac{\bar{I}}{2\pi\hat{s}} \hat{v}^2 \sum_{n=0}^{\infty} \frac{1}{(\hat{s} + 1)^{n+1}} \sum_{m=0}^n \binom{n}{m} \left(-\frac{\hat{k}}{\tanh(\hat{k})}\right)^m, \quad (\text{S.95})$$

$$\mathcal{L}[\hat{\phi}_0^b](\hat{k}, 1, \hat{s}) \approx \frac{\bar{I}}{2\pi\hat{s}^2} \hat{u}\hat{v} \frac{\hat{k}}{\sinh(\hat{k})} \sum_{n=0}^{\infty} \frac{1}{(\hat{s} + 1)^{n+1}} \sum_{m=0}^n \binom{n}{m} \left(-\frac{\hat{k}}{\tanh(\hat{k})}\right)^m, \quad (\text{S.96})$$

where we apply the binomial theorem to the  $\hat{k}$ -dependent term. Now that the series of  $\hat{s}$ -dependent and  $\hat{k}$ -dependent terms are separated, we can apply the inverse Laplace and Hankel transforms to each series independently.

The inverse Laplace transform of  $1/(\hat{s} + 1)^{n+1}$  is given by  $e^{-\hat{t}\hat{t}^n}/n!$ . For the inverse Hankel transform, we show in Appendix B that in the limit  $\hat{r} \gg 1$  (equivalently  $\hat{k} \ll 1$ )

$$\left(-\frac{\hat{k}}{\tanh(\hat{k})}\right)^m \leftrightarrow \frac{2\pi^2(\pi\hat{r})^{m-1}}{(m-1)!} K_0(\pi\hat{r}) (1 + \mathcal{O}(\hat{r}^{-1})), \quad (\text{S.97})$$

$$\frac{\hat{k}}{\sinh(\hat{k})} \left(-\frac{\hat{k}}{\tanh(\hat{k})}\right)^m \leftrightarrow \frac{2\pi^2(\pi\hat{r})^m}{m!} K_0(\pi\hat{r}) (1 + \mathcal{O}(\hat{r}^{-1})), \quad (\text{S.98})$$

where  $\leftrightarrow$  denotes the transform between Hankel and real spaces. When using these results to invert Eqs. (S.95) and (S.96), we must take only the leading order term in  $\hat{r}$  for consistency, which corresponds to  $m = n$ . This gives

$$\mathcal{L}^{-1}[\hat{s}\mathcal{L}[\hat{\phi}_0^b]](\hat{r}, 0, \hat{t}) = \frac{\bar{I}}{2\pi} \hat{v}^2 \frac{2\pi}{\hat{r}} K_0(\pi\hat{r}) e^{-\hat{t}} \sum_{n=1}^{\infty} \frac{(\pi\hat{r}\hat{t})^n}{n!(n-1)!} = \bar{I}\hat{v}^2 \sqrt{\frac{\pi\hat{t}}{\hat{r}}} K_0(\pi\hat{r}) e^{-\hat{t}} I_1(2\sqrt{\pi\hat{r}\hat{t}}), \quad (\text{S.99})$$

$$\mathcal{L}^{-1}[\hat{s}^2\mathcal{L}[\hat{\phi}_0^b]](\hat{r}, 1, \hat{t}) = \frac{\bar{I}}{2\pi} \hat{u}\hat{v} 2\pi^2 K_0(\pi\hat{r}) e^{-\hat{t}} \sum_{n=0}^{\infty} \frac{(\pi\hat{r}\hat{t})^n}{n!^2} = \bar{I}\pi\hat{u}\hat{v} K_0(\pi\hat{r}) e^{-\hat{t}} I_0(2\sqrt{\pi\hat{r}\hat{t}}), \quad (\text{S.100})$$

where we use the series representation for the modified Bessel function of the first kind  $I_0$  and its integrals. The additional factors of  $\hat{s}$  correspond to integrals in time, which can be performed by parts repeatedly to give

$$\bar{\phi}_0^b(\hat{r}, 0, \hat{t}) = \bar{I}\pi\hat{v}^2 e^{-\hat{t}} K_0(\pi\hat{r}) \sum_{n=2}^{\infty} \left(\frac{\hat{t}}{\pi\hat{r}}\right)^{n/2} I_n\left(2\sqrt{\pi\hat{r}\hat{t}}\right), \quad (\text{S.101})$$

$$\bar{\phi}_0^b(\hat{r}, 1, \hat{t}) = \bar{I}\pi\hat{u}\hat{v} e^{-\hat{t}} K_0(\pi\hat{r}) \sum_{n=2}^{\infty} (n-1) \left(\frac{\hat{t}}{\pi\hat{r}}\right)^{n/2} I_n\left(2\sqrt{\pi\hat{r}\hat{t}}\right). \quad (\text{S.102})$$

Since  $I_2(x), I_3(x), \dots$  is a decreasing sequence for any  $x > 0$ , the leading order for  $\hat{r} \gg \hat{t}$  is given by the  $n = 2$  term. From the boundary layer theory, this gives

$$\bar{\sigma}_0^m = \bar{\sigma}_0^e = \frac{\bar{I}(\chi+1)}{(\chi+2)^2} \frac{\hat{t}}{\hat{r}} e^{-\hat{t}} K_0(\pi\hat{r}) I_2\left(2\sqrt{\pi\hat{r}\hat{t}}\right), \quad (\text{S.103})$$

$$\bar{V}^M = \frac{2\bar{I}\chi(\chi+1)}{(\chi+2)^2} \frac{\hat{t}}{\hat{r}} e^{-\hat{t}} K_0(\pi\hat{r}) I_2\left(2\sqrt{\pi\hat{r}\hat{t}}\right). \quad (\text{S.104})$$

Equation (S.103) suggests that in the capacitive regime, the electrochemical response is characterized by symmetric charging of membrane and electrode surfaces.

### 3. Far field, diffusive regime ( $r > L, t > r/u$ )

The diffusive regime in the far field corresponds to  $t > r/u$ , or in dimensionless variables,  $\hat{t} > \hat{r}/\hat{u}$ . Equation (S.79) further suggests that diffuse behavior occurs at late times. To that end, from Eqs. (S.90) and (S.91), we can construct the full solution for the bulk electric potential using Eq. (S.69) as

$$\mathcal{L}[\hat{\phi}_0^b](\hat{k}, \hat{z}, \hat{s}) = \frac{\bar{I}}{2\pi\hat{s}} \frac{\hat{v}\hat{s} \sinh(\hat{k}(1-\hat{z})) + \hat{u}\hat{v}\hat{k} \cosh(\hat{k}(1-\hat{z}))}{(\hat{u}\hat{v}\hat{k}^2 + \hat{s}^2) \sinh(\hat{k}) + \hat{k}\hat{s} \cosh(\hat{k})}. \quad (\text{S.105})$$

Let us now consider the limit  $\hat{s} \rightarrow 0$  of Eq. (S.105), while keeping  $\hat{s}/\hat{k}^2$  finite. Accordingly

$$\mathcal{L}[\hat{\phi}_0^b](\hat{k}, \hat{z}, \hat{s}) \sim \frac{\bar{I}}{2\pi\hat{s}} \frac{1}{\hat{k}^2 + \frac{1}{\hat{u}\hat{v}}\hat{s}} + \mathcal{O}(\hat{s}^{-1}), \quad (\text{S.106})$$

which we recognize as constant in  $\hat{z}$ . Inverting the Laplace and Hankel transforms, the leading-order bulk potential assumes the form

$$\bar{\phi}_0^b(\hat{r}, \hat{z}, \hat{t}) \sim \hat{D}_{\text{eff}} \bar{I} \int_0^{\hat{t}} \frac{e^{-\frac{\hat{r}^2}{4\hat{D}_{\text{eff}}\hat{\tau}}}}{4\pi\hat{D}_{\text{eff}}\hat{\tau}} d\hat{\tau} = -\frac{\bar{I}}{4\pi} \text{Ei}\left(-\frac{\hat{r}^2}{4\hat{D}_{\text{eff}}\hat{t}}\right), \quad (\text{S.107})$$

where  $\text{Ei}(x) \equiv -\int_{-x}^{\infty} e^{-\alpha}/\alpha d\alpha$  is the exponential integral [8] and  $\hat{D}_{\text{eff}} = \hat{u}\hat{v}$  is the effective diffusivity. In dimensional form,

$$D_{\text{eff}} = \hat{D}_{\text{eff}} \frac{L^2}{\tau_C} = \hat{u}\hat{v} \frac{L^2}{\hat{u} \frac{L\lambda_D}{D}} = \hat{v} \frac{L}{\lambda_D} D = \frac{1+\chi}{2+\chi} \frac{L}{\lambda_D} D, \quad (\text{S.108})$$

as advertised in the main text.

The integrand in Eq. (S.107) is the Green's function for the diffusion of an instantaneous unit line source of a solute at the origin [9]. Hence, at long times the bulk potential behaves as though it diffuses radially outward from a continuous line source of strength  $\hat{D}_{\text{eff}}\bar{I}$ . Because Eq. (S.107) is independent of  $\hat{z}$ , axial variations disappear once  $\hat{t} \gg 1$ .

The uniformity in  $\hat{z}$  yields a simple governing equation for the late-time diffusive behavior. Integrating Eq. (S.62) over  $\hat{z}$  we get

$$0 = \frac{1}{\hat{r}} \frac{\partial}{\partial \hat{r}} \left( \hat{r} \frac{\partial \bar{\phi}_0^b}{\partial \hat{r}} \right) + \left[ \frac{\partial \bar{\phi}_0^b}{\partial \hat{z}} \right]_{\hat{z}=0}^{\hat{z}=1}, \quad (\text{S.109})$$

where  $\bar{\psi}_0^b(\hat{r}, \hat{t}) \equiv \int_0^1 \bar{\phi}_0^b(\hat{r}, \hat{z}, \hat{t}) d\hat{z}$  is the  $\hat{z}$ -averaged bulk potential. Applying the boundary conditions (S.63) and (S.64), we get

$$0 = \frac{1}{\hat{r}} \frac{\partial}{\partial \hat{r}} \left( \hat{r} \frac{\partial \bar{\psi}_0^b}{\partial \hat{r}} \right) - (2 + \chi) \left( \frac{\partial \bar{\phi}_0^b}{\partial \hat{t}} \Big|_{\hat{z}=1} + \frac{1}{1 + \chi} \frac{\partial \bar{\phi}_0^b}{\partial \hat{t}} \Big|_{\hat{z}=0} \right) + \bar{I} \frac{\delta(\hat{r})}{2\pi \hat{r}}. \quad (\text{S.110})$$

At late times, the bulk electric field in the axial direction relaxes so that  $\bar{\phi}_0^b|_{\hat{z}=0} \approx \bar{\phi}_0^b|_{\hat{z}=1} \approx \bar{\psi}_0^b(\bar{r}, \bar{t})$ . Consequently, we have

$$0 = \frac{\partial \bar{\psi}_0^b}{\partial \hat{t}} - \hat{D}_{\text{eff}} \frac{1}{\hat{r}} \frac{\partial}{\partial \hat{r}} \left( \hat{r} \frac{\partial \bar{\psi}_0^b}{\partial \hat{r}} \right) - \hat{D}_{\text{eff}} \bar{I} \frac{\delta(\hat{r})}{2\pi \hat{r}}, \quad (\text{S.111})$$

which encapsulates the late-time behavior: the averaged potential spreads purely by radial diffusion with diffusivity  $\hat{D}_{\text{eff}}$ , driven continuously by the line source of strength  $\bar{I}$ . As one might expect for consistency, the explicit solution Eq. (S.107) satisfies Eq. (S.111).

At long times  $\hat{t} > \hat{r}^2/4\hat{D}_{\text{eff}}$ , the solution to Eq. (S.111) predicts that  $\bar{\psi}_0^b \sim \bar{V}^M \propto \log(4\hat{D}_{\text{eff}}\hat{t}/\hat{r}^2)$ . The diffusive regime first emerges at  $\hat{r} \sim 1$ , when  $\hat{t} \sim 1$ , and then spreads both inward and outward. At sufficiently late times, it also overtakes the near-field profile (Eq. (S.89)) for  $r < L$ . Thus, for blocking electrodes,  $\bar{V}^M$  grows logarithmically in time at every fixed radius.

This logarithmic divergence at long times is seemingly at odds with the steady-state behavior described in Sec. V.1. However, this discrepancy arises because the limits  $\hat{k} \rightarrow \infty$  and  $\hat{s} \rightarrow 0$  (or equivalently,  $\hat{r} \rightarrow 0$  and  $\hat{t} \rightarrow \infty$ ) do not commute. By considering  $\hat{k} \rightarrow \infty$  in Sec. V.1, we effectively took the limit as  $\hat{r} \rightarrow 0$  for fixed, finite time  $\hat{t}$ . In this setting, however large  $\hat{t}$  may be, there is always a sufficiently small value of  $\hat{r}$  where the monopolar behavior is recovered. This is evident in the expression for the crossover time  $\hat{t}^*(\hat{r})$  between the monopolar and diffusive behavior

$$\hat{t}^* = \hat{r}^2 \exp\left(\frac{1}{\hat{r}} - 1\right), \quad (\text{S.112})$$

which clearly shows that as  $\hat{r} \rightarrow 0$ ,  $\hat{t}^* \rightarrow \infty$ . This singularity is the reason why the two limits do not commute.

The divergent behavior at long times is also confirmed when directly considering the limit as  $\hat{t} \rightarrow \infty$  of the exact solutions Eqs. (S.80) and (S.81). The Hankel transform is ill-defined because of the divergent behavior. Finally, both the monopolar and diffusive regimes may be reconciled by noting that in the joint limit of  $\hat{r} \rightarrow 0$  and  $\hat{t} \rightarrow \infty$ , Eq. (S.112) defines a line separating the logarithmically growing, diffusive behavior from the steady monopolar behavior.

## VI. Late time solutions: Faradaic electrodes

With ideal Faradaic electrodes, the charge-balance condition at the electrode surface changes to satisfy Eq. (S.14-C). Because the electrostatic boundary conditions are otherwise identical to those for blocking electrodes, the early-time dynamics (described by using the point charge approximation in Sec. IV) are unchanged. We therefore focus on the late-time behaviour and use singular-perturbation methods to obtain uniformly valid solutions for the case of perfect Faradaic electrodes.

For the outer (bulk) region, the asymptotic expansions (S.17) and (S.18) in limit of  $\eta \rightarrow 0$  yields the same governing equations (S.19) and (S.21). The outer solutions directly satisfy the boundary conditions Eqs. (S.12-C) and (S.14-C), because no boundary layer develops on the electrode surface. The bulk equations then read

$$\bar{\rho}_n^b(\hat{\mathbf{x}}, \hat{t}) = 0 \quad (n = 0, 1, 2, \dots), \quad (\text{S.113})$$

$$\hat{\nabla}^2 \bar{\phi}_n^b = 0 \quad (n = 0, 1, 2, \dots), \quad (\text{S.114})$$

$$\bar{\phi}_n^b|_{\hat{z}=1} = 0 \quad (n = 0, 1, 2, \dots), \quad (\text{S.115})$$

prohibiting free charge in the bulk. The electric potential remains harmonic, as in the case of blocking electrodes.

Near the membrane ( $\hat{z} = 0$ ) the analysis of Sec. III.2 remains the same. The leading-order inner solutions are still given by Eqs. (S.32) and (S.33). Because only the two membrane-side diffuse layers are now present ( $n_D = 2$ ), the boundary condition Eq. (S.41) becomes

$$\left. \frac{\partial \bar{\phi}_0^b}{\partial \hat{t}} \right|_{\hat{z}=0} = \bar{I} \frac{\delta(\hat{r})}{2\pi \hat{r}} + \left. \frac{\partial \bar{\phi}_0^b}{\partial \hat{z}} \right|_{\hat{z}=0} . \quad (\text{S.116})$$

Applying the Laplace transform in  $\hat{t}$  and the Hankel transform in  $\hat{r}$  to Eqs. (S.114), (S.115), and (S.116) gives

$$\frac{\partial^2 \mathcal{L}[\hat{\phi}_0^b]}{\partial \hat{z}^2} - \hat{k}^2 \mathcal{L}[\hat{\phi}_0^b] = 0 , \quad (\text{S.117})$$

$$\mathcal{L}[\hat{\phi}_0^b] \Big|_{\hat{z}=1} = 0 , \quad (\text{S.118})$$

$$\hat{s} \mathcal{L}[\hat{\phi}_0^b] \Big|_{\hat{z}=0} = \frac{\bar{I}}{2\pi \hat{s}} + \left. \frac{\partial \mathcal{L}[\hat{\phi}_0^b]}{\partial \hat{z}} \right|_{\hat{z}=0} . \quad (\text{S.119})$$

Solving yields

$$\mathcal{L}[\hat{\phi}_0^b](\hat{k}, \hat{z}, \hat{s}) = \frac{\bar{I}}{2\pi \hat{s}} \frac{\sinh(\hat{k}(1-\hat{z}))}{\hat{s} \sinh \hat{k} + \hat{k} \cosh \hat{k}} . \quad (\text{S.120})$$

The solution has a simple pole  $\hat{s}_F = -\hat{k}/\tanh \hat{k}$ , whose magnitude controls the timescale. For  $\hat{k} \gg 1$ ,  $\hat{s}_F \sim -\hat{k}$  (front-like radial propagation); conversely, for  $\hat{k} \ll 1$ ,  $\hat{s}_F \sim -1$  (global relaxation on the capacitive timescale  $\tau_C$ ). Inverting the Laplace transform in (S.120) gives

$$\hat{\phi}_0^b(\hat{k}, \hat{z}, \hat{t}) = \frac{\bar{I}}{2\pi} \frac{\sinh(\hat{k}(1-\hat{z}))}{\hat{k} \cosh \hat{k}} \left( 1 - e^{-\frac{\hat{k}}{\tanh \hat{k}} \hat{t}} \right) . \quad (\text{S.121})$$

## 1. Near-field ( $r < L$ ) solution

We again consider the short wavelength limit  $\hat{k} \gg 1/(1-\hat{z}) \geq 1$  or  $\hat{r} \ll 1-\hat{z}$  (i.e., the distance to the electrode is much greater than the distance to the axis of symmetry). In this limit Eq. (S.121) simplifies to

$$\hat{\phi}_0^b(\hat{k}, \hat{z}, \hat{t}) = \frac{\bar{I}}{2\pi} \frac{e^{-\hat{k}\hat{z}}}{\hat{k}} \left( 1 - e^{-\hat{k}\hat{t}} \right) . \quad (\text{S.122})$$

Inverting the Hankel transform yields the real-space potential

$$\bar{\phi}_0^b(\hat{r}, \hat{z}, \hat{t}) = \frac{\bar{I}}{2\pi} \left( \frac{1}{\sqrt{\hat{r}^2 + \hat{z}^2}} - \frac{1}{\sqrt{\hat{r}^2 + (\hat{z} + \hat{t})^2}} \right) , \quad (\text{S.123})$$

valid when  $\hat{r} \ll 1-\hat{z}$ . The corresponding areal charge density and transmembrane potential are

$$\bar{\sigma}_0^m(\hat{r}, \hat{t}) = \frac{\bar{I}}{2\pi(1+\chi)} \left( \frac{1}{\hat{r}} - \frac{1}{\sqrt{\hat{r}^2 + \hat{t}^2}} \right) , \quad (\text{S.124})$$

$$\bar{V}^M(\hat{r}, \hat{t}) = \frac{\bar{I}\chi}{\pi(1+\chi)} \left( \frac{1}{\hat{r}} - \frac{1}{\sqrt{\hat{r}^2 + \hat{t}^2}} \right) . \quad (\text{S.125})$$

which reproduce the near-field expressions of Ref. [5] corresponding to monopolar and dipolar regions. Moreover, constructing the uniformly valid solutions for the charge density and the electric potential using Eqs. (S.54) and (S.55) recover the results of Ref. [5] for the charge density and the electric potential. Comparison of the Faradaic results with the unbounded results is shown in Fig. S4(a).

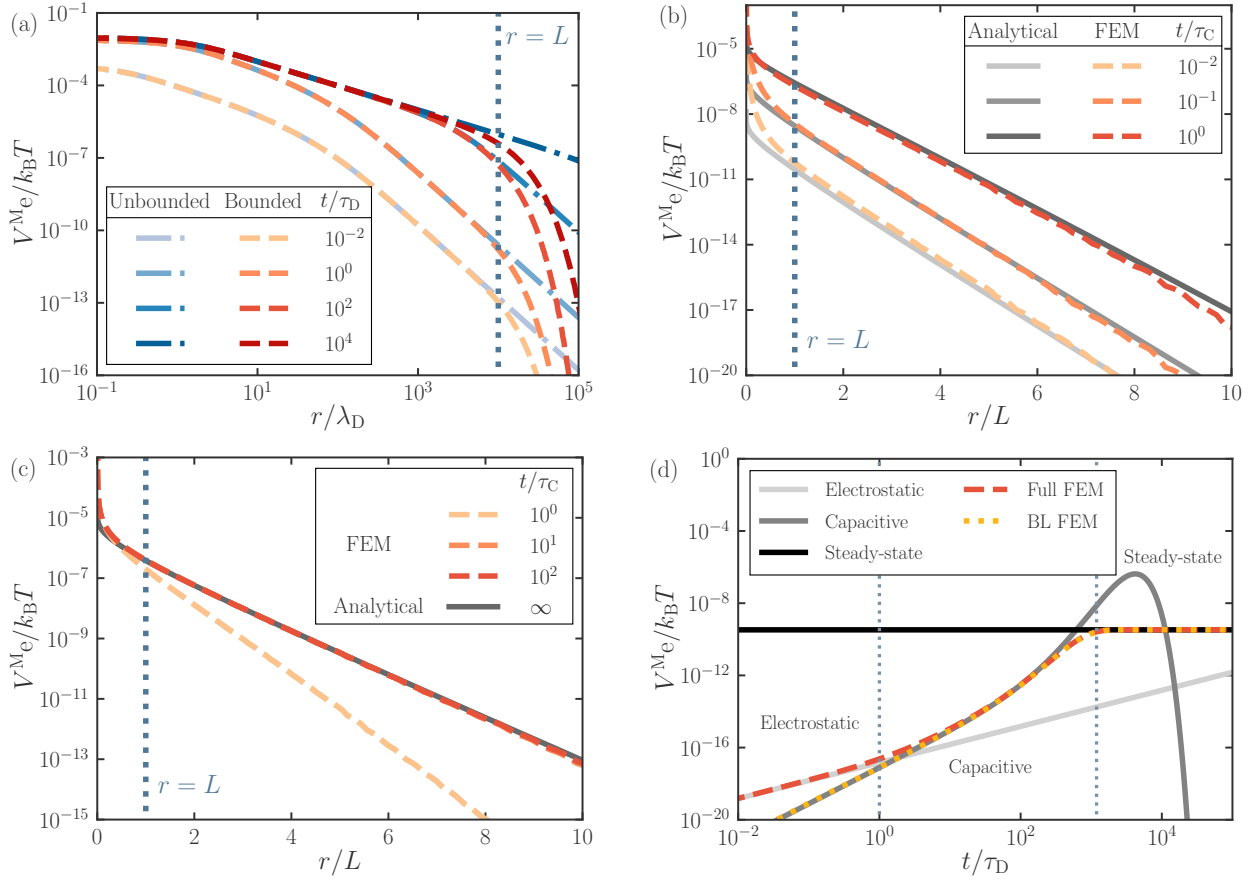

Figure S4: Comparison of FEM results for Faradaic electrodes with analytical solutions. (a) Near-field region compared with FEM solutions to unbounded electrolyte from Ref. [5] shows that they are equivalent at  $r < L$ . (b) Far-field region at times  $t \leq \tau_C$  compared with capacitive solution. (c) Far-field region at times  $t \geq \tau_C$  compared with steady-state solution. (d) Data for  $r = 5L$  in time showing the agreement of the analytical solutions in the electrostatic, capacitive, and steady-state regions. All simulations were performed with parameters as in Fig. 3 of the main text.

## 2. Far-field, capacitive regime ( $r > L$ , $\tau_D < t < r/v$ )

In the far field ( $\hat{k} \ll 1$ ), the Laplace-Hankel expression in Eq. (S.120) reduces to

$$\mathcal{L}[\hat{\phi}_0^b](\hat{k}, \hat{z}, \hat{s}) = \frac{\bar{I}}{2\pi\hat{s}} \frac{\sinh(\hat{k}(1-\hat{z}))}{\sinh(\hat{k})} \frac{1}{\hat{s} + \frac{\hat{k}}{\tanh(\hat{k})}}. \quad (\text{S.126})$$

At the surface  $\hat{z} = 0$ ,

$$\mathcal{L}[\hat{\phi}_0^b](\hat{k}, 0, \hat{s}) = \frac{\bar{I}}{2\pi\hat{s}} \frac{1}{\hat{s} + \frac{\hat{k}}{\tanh(\hat{k})}}, \quad (\text{S.127})$$

which is identical to the blocking electrode expression Eq. (S.92) but with  $\hat{v} = 1$ . Repeating the analysis of Sec. V.2 based on the Laurent expansion yields for  $\hat{r} \gg 1$

$$\hat{\phi}_0^b(\hat{r}, 0, \hat{t}) = \bar{I}\pi e^{-\hat{t}} K_0(\pi\hat{r}) \sum_{n=2}^{\infty} \left( \frac{\hat{t}}{\pi\hat{r}} \right)^{n/2} I_n \left( 2\sqrt{\pi\hat{r}\hat{t}} \right), \quad (\text{S.128})$$

and keeping the leading term for  $\hat{r} \gg \hat{t}$  results in

$$\bar{\sigma}_0^m = \frac{\bar{I}}{\chi+1} \frac{\hat{t}}{\hat{r}} e^{-\hat{t}} K_0(\pi\hat{r}) I_2 \left( 2\sqrt{\pi\hat{r}\hat{t}} \right), \quad (\text{S.129})$$

$$\bar{V}^M = \frac{2\bar{I}\chi}{\chi+1} \frac{\hat{t}}{\hat{r}} e^{-\hat{t}} K_0(\pi\hat{r}) I_2 \left( 2\sqrt{\pi\hat{r}\hat{t}} \right). \quad (\text{S.130})$$

Figure S4(b) compares this result for  $V^M$  with the numerical solution.

## 3. Steady-state solution

Unlike the case of blocking electrodes, the system admits a steady state with Faradaic electrodes. Because the magnitude of the pole  $|\hat{s}_F| < 1$  for all  $\hat{k}$ , the relaxation to steady state occurs when  $t \gg \tau_C$ . From Eq. (S.121), the steady state solution is given by

$$\hat{\phi}_{0,ss}^b(\hat{k}, \hat{z}) = \frac{\bar{I}}{2\pi} \frac{\sinh(\hat{k}(1-\hat{z}))}{\hat{k} \cosh \hat{k}}. \quad (\text{S.131})$$

Using the Taylor expansion  $1/\cosh \hat{k} = 2e^{-\hat{k}} \sum_{n=0}^{\infty} (-1)^n e^{-2n\hat{k}}$ , inverting term-by-term yields the image-charge representation of the steady-state solution,

$$\bar{\phi}_{0,ss}^b(\hat{r}, \hat{z}) = \frac{\bar{I}}{2\pi} \sum_{m=-\infty}^{\infty} \frac{(-1)^m}{\sqrt{\hat{r}^2 + (\hat{z} - 2m)^2}}, \quad (\text{S.132})$$

or equivalently, from Appendix A Eq. (S.165), the spectral form,

$$\bar{\phi}_{0,ss}^b(\hat{r}, \hat{z}) = \frac{\bar{I}}{\pi} \sum_{n=1}^{\infty} K_0 \left( \frac{2n-1}{2} \pi \hat{r} \right) \cos \left( \frac{2n-1}{2} \pi \hat{z} \right). \quad (\text{S.133})$$

For  $\hat{r} \gg 1$ , the leading mode dominates:

$$\bar{\phi}_{0,ss}^b(\hat{r}, \hat{z}) \approx \frac{\bar{I}}{\pi} K_0 \left( \frac{\pi}{2} \hat{r} \right) \cos \left( \frac{\pi}{2} \hat{z} \right). \quad (\text{S.134})$$

Figure S4(c) compares the result for  $V^M$  with the numerical solution at times  $t \geq \tau_C$ . Also, Fig. S4(d) shows the time evolution of  $V^M$  and the transitions between the three asymptotic regimes identified: electrostatic, capacitive, and steady-state.

## VII. External current

As argued in the main text, to ensure that the electrodes remain at a fixed potential, they must develop an induced surface charge during the electrochemical response. The adjustment of surface charge may involve an external current  $I^{\text{ext}}$  through the wire that connects the two electrodes to a potentiostat, as illustrated in Fig. 7 of the main text. We now derive  $I^{\text{ext}}$  for both blocking and Faradaic electrodes.

From a global balance on the electrode at  $z = L$ , adjustments in surface charge arise due to the external current or Faradaic fluxes from the electrolyte

$$\int_{S^e} \frac{\partial \sigma_{\text{ind}}^e}{\partial t} da = -I^{\text{ext}} + \int_{S^e} \mathbf{e}_z \cdot \mathbf{j}_\rho da, \quad (\text{S.135})$$

where  $S^e$  is the electrode surface,  $\sigma_{\text{ind}}^e$  is the induced surface charge density,  $\mathbf{j}_\rho$  is the charge flux, and  $da$  is the area element. Gauss's law relates  $\sigma_{\text{ind}}^e$  to the normal component of the electric field

$$\sigma_{\text{ind}}^e = \epsilon \left. \frac{\partial \phi^e}{\partial z} \right|_{z=L}. \quad (\text{S.136})$$

Nondimensionalizing Eqs. (S.135) and (S.136) yields

$$\int_{\hat{S}^e} \frac{\partial \bar{\sigma}_{\text{ind}}^e}{\partial \hat{t}} d\hat{a} = -\hat{u} \bar{I}^{\text{ext}} + \eta^{-1} \int_{\hat{S}^e} \mathbf{e}_{\hat{z}} \cdot \bar{\mathbf{j}}_\rho d\hat{a}, \quad (\text{S.137})$$

$$\bar{\sigma}_{\text{ind}}^e = \eta \left. \frac{\partial \bar{\phi}^e}{\partial \hat{z}} \right|_{\hat{z}=1}, \quad (\text{S.138})$$

where the dimensionless variables are defined as  $\bar{\sigma}_{\text{ind}}^e \equiv \sigma_{\text{ind}}^e / (2eC^0 \lambda_D)$  and  $\bar{I}^{\text{ext}} \equiv I^{\text{ext}} / (\phi_T L g)$ . We keep the electrode area  $A^e$  finite, but with the lateral dimensions of the electrodes being much larger than  $L$  so that edge effects are negligible, and the infinite electrode solutions can be used to estimate the external current. Since the “current-driven” and “voltage-driven” problems are linearly decomposable (see Eq. (S.15)), we treat the contributions from each separately in the following subsections and superimpose them at the end. In what follows, we drop the superscript ‘e’ from the surface charge and potential symbols.

### 1. Blocking electrodes ( $n_D = 4$ , $\hat{u} = (2 + \chi)^{-1}$ , $\hat{v} = 1 - \hat{u}$ )

Blocking surfaces do not permit ionic flux, so the second term on the RHS of (S.137) vanishes

$$\int_{\hat{S}^e} \frac{\partial \bar{\sigma}_{\text{ind}}}{\partial \hat{t}} d\hat{a} = -\hat{u} \bar{I}^{\text{ext}}. \quad (\text{S.139})$$

By combining Eqs. (S.139) and (S.138), we obtain

$$\bar{I}^{\text{ext}} = -\frac{\eta}{\hat{u}} \frac{\partial}{\partial \hat{t}} \int_{\hat{S}^e} \left. \frac{\partial \bar{\phi}}{\partial \hat{z}} \right|_{\hat{z}=1} d\hat{a}, \quad (\text{S.140})$$

where the electric potential  $\bar{\phi}$  is decomposed by the contributions from the transmembrane ionic current  $\bar{\phi}^C$  and applied voltage  $\bar{\phi}^V$  following Eq. (S.15). We now evaluate each of these contributions.

#### (a). Contribution from $\bar{\phi}^C$

Near the electrode, the potential is described by the inner solution  $\bar{\phi}_0^e(\hat{r}, \hat{z}', \hat{t})$  in Eq. (S.49) at leading order. Since the potential decays exponentially with radial distance for  $r \gg L$ , the current-driven contribution to the integral over the electrode surface in Eq. (S.140) can be approximated as

$$\int_{\hat{S}^e} \left. \frac{\partial \bar{\phi}^C}{\partial \hat{z}} \right|_{\hat{z}=1} d\hat{a} \approx \int_0^\infty d\hat{r} 2\pi \hat{r} \left. \frac{\partial \bar{\phi}^C}{\partial \hat{z}} \right|_{\hat{z}=1}. \quad (\text{S.141})$$

The right-hand side can be calculated exactly by using a property of the Hankel transform that the limit  $\hat{k} \rightarrow 0$  gives an integral of the original function over a plane (with a factor of  $2\pi$ ). From Eqs. (S.49) and (S.71)

$$\hat{\phi}_0^C(\hat{k}, \hat{z}', \hat{t}) \equiv \int_0^\infty d\hat{r} \hat{r} \bar{\phi}_0^C(\hat{r}, \hat{z}', \hat{t}) J_0(\hat{k}\hat{r}) = \hat{\phi}_0^b(\hat{k}, 1, \hat{t}) (1 - e^{-\hat{z}'}), \quad (\text{S.142})$$

where  $\hat{\phi}_0^b(\hat{k}, 1, \hat{t})$  is given by Eq. (S.81). Now, we take a limit  $\hat{k} \rightarrow 0$  to obtain the integral over the surface as

$$\int_0^\infty d\hat{r} 2\pi\hat{r} \left. \frac{\partial \bar{\phi}^C}{\partial \hat{z}} \right|_{\hat{z}=1} = -2\pi\eta^{-1} \lim_{\hat{k} \rightarrow 0} \hat{\phi}_0^b(\hat{k}, 1, \hat{t}) e^{-\hat{z}'}, \quad (\text{S.143})$$

where the factor of  $\eta^{-1}$  emerges from the chain rule, i.e.  $\partial \hat{z}' / \partial \hat{z} = -\eta^{-1}$ . Evaluating Eq. (S.143) at  $\hat{z} = 1$ , or equivalently  $\hat{z}' = 0$ , Eq. (S.141) yields the external current as

$$\bar{I}^{\text{ext}} = \left(1 + \frac{\hat{u}}{\hat{v}}\right)^{-1} \bar{I}(1 - e^{-\hat{t}}) = \frac{1 + \chi}{2 + \chi} \bar{I}(1 - e^{-\hat{t}}) = \hat{v} \bar{I}(1 - e^{-\hat{t}}). \quad (\text{S.144})$$

Thus,  $\bar{I}^{\text{ext}}$  only carries a fraction of the transmembrane current  $\bar{I}$  even at long times. The remainder continues to accumulate as areal charge in the membrane-side and electrode-side boundary layers.

### (b). Contribution from $\bar{\phi}^V$

The linear dynamics of the charge density and potential for the voltage-driven problem is given by Ref. [4] as

$$\bar{\rho}^V(\hat{z}, \hat{t}) = \bar{V} \hat{u} \left( e^{-\hat{z}/\eta} - e^{-(1-\hat{z})/\eta} \right) (1 - e^{-\hat{t}}), \quad (\text{S.145})$$

$$\bar{\phi}^V(\hat{z}, \hat{t}) = \bar{V} \left[ 1 - (1 - \hat{z})e^{-\hat{t}} - \hat{u} \left( 1 + e^{-\hat{z}/\eta} - e^{-(1-\hat{z})/\eta} \right) (1 - e^{-\hat{t}}) \right], \quad (\text{S.146})$$

when  $\hat{t} \gg \tau_D / \tau_C$ . From Eq. (S.140), we can calculate the voltage-driven contribution to the external current at leading order as

$$\bar{I}^{\text{ext}} = -\bar{V} \hat{A}^e e^{-\hat{t}}, \quad (\text{S.147})$$

indicating that the external current required to maintain the applied voltage exponentially decays with the capacitive time scale.

### (c). Linear superposition

Summing Eqs. (S.144) and (S.147) yields

$$\bar{I}^{\text{ext}} = \hat{v} \bar{I}(1 - e^{-\hat{t}}) - \bar{V} \hat{A}^e e^{-\hat{t}}, \quad (\text{S.148})$$

for the net external current due to both stimuli.

## 2. Ideal Faradaic electrode ( $n_D = 2$ , $\hat{u} = (1 + \chi)^{-1}$ , $\hat{v} = 1$ )

In this case, the electrodes supply or withdraw charges to maintain  $\rho = 0$  at the electrode-electrolyte interface. Combining Eqs. (S.137) and (S.138) the global charge balance on the electrode is

$$\bar{I}^{\text{ext}} = -\frac{\eta}{\hat{u}} \frac{\partial}{\partial \hat{t}} \int_{\hat{S}^e} \left. \frac{\partial \bar{\phi}}{\partial \hat{z}} \right|_{\hat{z}=1} d\hat{a} + \frac{1}{\hat{u}\eta} \int_{\hat{S}^e} \mathbf{e}_z \cdot \bar{\mathbf{j}}_\rho d\hat{a}, \quad (\text{S.149})$$

where  $\hat{u} \equiv (n_D/2 + \chi)^{-1} = (1 + \chi)^{-1}$ . Since the bulk charge density vanishes at leading order, the charge flux at the electrode surface  $\bar{\mathbf{j}}_\rho|_{\hat{z}=1} \sim -\hat{u}\eta \bar{\nabla} \bar{\phi}|_{\hat{z}=1}$  from Eq. (S.6). Thus

$$\bar{I}^{\text{ext}} = -\frac{\eta}{\hat{u}} \frac{\partial}{\partial \hat{t}} \int_{\hat{S}^e} \left. \frac{\partial \bar{\phi}}{\partial \hat{z}} \right|_{\hat{z}=1} d\hat{a} - \int_{\hat{S}^e} \left. \frac{\partial \bar{\phi}}{\partial \hat{z}} \right|_{\hat{z}=1} d\hat{a}. \quad (\text{S.150})$$

Equation (S.150) shows that for Faradaic electrodes, the dominant contribution to  $\bar{I}^{\text{ext}}$  arises from the second term, representing the charge flux from the electrolyte. To proceed further, we need to calculate the integral  $\int_{\hat{S}^e} (\partial \bar{\phi} / \partial \hat{z})|_{\hat{z}=1} d\hat{a}$ . As before, we will evaluate the contributions from  $\bar{\phi}^C$  and  $\bar{\phi}^V$  separately.

### (a). Contribution from $\bar{\phi}^C$

Recall for Faradaic electrodes that  $\bar{\phi}^C$  at the membrane surface is given by the bulk potential  $\bar{\phi}^b$ . The Hankel transform of the bulk potential

$$\hat{\phi}_0^b(\hat{k}, \hat{z}, \hat{t}) \equiv \int_0^\infty d\hat{r} \hat{r} \bar{\phi}_0^b(\hat{r}, \hat{z}', \hat{t}) J_0(\hat{k}\hat{r}) = \frac{\bar{I}}{2\pi} \frac{\sinh(\hat{k}(1-\hat{z}))}{\hat{k} \cosh \hat{k}} \left(1 - e^{-\frac{\hat{k}}{\tanh \hat{k}} \hat{t}}\right), \quad (\text{S.151})$$

where we use the expression in Eq. (S.121) for the second equality. In the limit  $\hat{k} \rightarrow 0$

$$\int_0^\infty d\hat{r} \hat{r} \bar{\phi}_0^b(\hat{r}, \hat{z}', \hat{t}) = \frac{\bar{I}}{2\pi} (1-\hat{z}) \left(1 - e^{-\hat{t}}\right). \quad (\text{S.152})$$

Because the potential exponentially decays in radial direction, for a sufficiently large electrode at leading order

$$\int_{\hat{S}^e} \frac{\partial \bar{\phi}^C}{\partial \hat{z}} \Big|_{\hat{z}=1} d\hat{a} \approx \int_0^\infty d\hat{r} 2\pi \hat{r} \frac{\partial \bar{\phi}^C}{\partial \hat{z}} \Big|_{\hat{z}=1} = -\bar{I} \left(1 - e^{-\hat{t}}\right). \quad (\text{S.153})$$

From Eq. (S.150), the external current

$$\bar{I}^{\text{ext}} = \bar{I} \left(1 - e^{-\hat{t}}\right) + \mathcal{O}(\eta), \quad (\text{S.154})$$

indicating that beyond the capacitive time scale, the external current equals the transmembrane current.

### (b). External current to maintain the applied voltage

The leading order uniform solution to the charge density and potential for the voltage-driven problem is given by

$$\bar{\rho}^V(\hat{z}, \hat{t}) = \bar{V} \hat{u} e^{-\hat{z}/\eta} \left(1 - e^{-\hat{t}}\right), \quad (\text{S.155})$$

$$\bar{\phi}^V(\hat{z}, \hat{t}) = \bar{V} \left[1 - (1-\hat{z})e^{-\hat{t}} - \hat{u} e^{-\hat{z}/\eta} \left(1 - e^{-\hat{t}}\right)\right], \quad (\text{S.156})$$

which we obtain from the formulas of Ref. [4] by “removing” the electrode-side diffuse layers. From Eq. (S.150), the leading order current from the voltage-driven contribution is

$$\bar{I}^{\text{ext}} = \bar{V} \hat{A}^e e^{-\hat{t}} + \mathcal{O}(\eta). \quad (\text{S.157})$$

### (c). Linear superposition

Summing Eqs. (S.154) and (S.157) yields the total current under both stimuli as

$$\bar{I}^{\text{ext}} = \bar{I} \left(1 - e^{-\hat{t}}\right) + \bar{V} \hat{A}^e e^{-\hat{t}}. \quad (\text{S.158})$$

## References

- [1] P. Debye and E. Hückel, *Physikalische Zeitschrift* **24**, 185 (1923).
- [2] M. Gouy, *Journal de Physique Théorique et Appliquée* **9**, 457–468 (1910).
- [3] M. Z. Bazant, K. Thornton, and A. Ajdari, *Physical Review E* **70**, 021506 (2004).
- [4] J. Farhadi, J. B. Fernandes, K. Shekhar, and K. K. Mandadapu, *Physical Review E* **111**, 064412 (2025).
- [5] H. Row, J. B. Fernandes, K. K. Mandadapu, and K. Shekhar, *Physical Review Research* **7**, 013185 (2025).

- [6] P. Debye and H. Falkenhagen, *Zeitschrift für Elektrochemie und angewandte physikalische Chemie* **34**, 562 (1928).
- [7] M. Abramowitz and I. A. Stegun, *Handbook of Mathematical Functions with Formulas, Graphs, and Mathematical Tables* (US Government Printing Office, 1968).
- [8] G. B. Arfken, H. J. Weber, and F. E. Harris, *Mathematical Methods for Physicists: A Comprehensive Guide* (Academic Press, 2011).
- [9] J. Crank, *The Mathematics of Diffusion* (Oxford University Press, 1979).
- [10] J. Shen, T. Tang, and L.-L. Wang, *Spectral methods: algorithms, analysis and applications*, Vol. 41 (Springer Science & Business Media, 2011).
- [11] M. Majic, arXiv preprint arXiv:2001.10651 (2020).
- [12] DLMF, “*NIST Digital Library of Mathematical Functions*,” <https://dlmf.nist.gov/>, Release 1.2.4 of 2025-03-15, f. W. J. Olver, A. B. Olde Daalhuis, D. W. Lozier, B. I. Schneider, R. F. Boisvert, C. W. Clark, B. R. Miller, B. V. Saunders, H. S. Cohl, and M. A. McClain, eds.

## A. Image charge transformations

We frequently need to inter-convert infinite sums of rational functions arising in image-charge representations into infinite sums of eigenfunction expansions (e.g., Eq. (S.58)  $\leftrightarrow$  Eq. (S.59)) [10]. This section derives such relationships, which are motivated by considering the electric potentials of point charges placed between parallel conducting discs [11].

For every positive integer  $p$  define

$$f(r, z) = \sum_{m=-\infty}^{\infty} \frac{1}{((2m+z)^2 + r^2)^{p+\frac{1}{2}}} . \quad (\text{S.159})$$

It can be easily seen by reindexing  $m \rightarrow m+1$  that the function  $f$  is periodic in  $z$  with period 2. Therefore, we can expand  $f$  in the Fourier basis  $\{\cos(n\pi z), \sin(n\pi z) : n \in \{0, 1, 2, \dots\}\}$  as

$$f(r, z) = \frac{1}{2} A_0(r) + \sum_{n=1}^{\infty} [A_n(r) \cos(n\pi z) + B_n(r) \sin(n\pi z)] . \quad (\text{S.160})$$

Next, by reindexing  $m \rightarrow -m$  in Eq. (S.159), we observe that  $f$  is even in  $z$ . Therefore, all sine contributions vanish,  $B_n = 0$ . The cosine coefficients can be calculated from the orthonormality of the basis functions

$$A_n(r) = \int_{-1}^1 f(r, z) \cos(n\pi z) dz . \quad (\text{S.161})$$

Substituting Eq. (S.159) and simplifying

$$\begin{aligned} A_n(r) &= \int_{-1}^1 \sum_{m=-\infty}^{\infty} \frac{\cos(n\pi z)}{((2m+z)^2 + r^2)^{p+\frac{1}{2}}} dz \\ &= \sum_{m=-\infty}^{\infty} \int_{-1}^1 \frac{\cos(n\pi z)}{((2m+z)^2 + r^2)^{p+\frac{1}{2}}} dz && \text{(exchanging sum and integral)} \\ &= \sum_{m=-\infty}^{\infty} \int_{2m-1}^{2m+1} \frac{\cos(n\pi y - 2nm\pi)}{(y^2 + r^2)^{p+\frac{1}{2}}} dy && \text{(change of variable } y = 2m + z) \\ &= \sum_{m=-\infty}^{\infty} \int_{2m-1}^{2m+1} \frac{\cos(n\pi y)}{(y^2 + r^2)^{p+\frac{1}{2}}} dy && \text{(using periodicity and } m, n \in \mathbb{Z}) \end{aligned}$$

$$= \int_{-\infty}^{\infty} \frac{\cos(n\pi y)}{(y^2 + r^2)^{p+\frac{1}{2}}} dy \quad (\text{integral telescopes}) .$$

For  $n = 0$ , the integral is straight forward to compute and yields  $(2/r^2)^p (p-1)!/(2p-1)!!$ . For  $n \geq 1$ , we apply Basset's integral formula [12, (10.32.11)],

$$K_\nu(xz) = \frac{\Gamma(\nu + \frac{1}{2})(2z)^\nu}{\sqrt{\pi}x^\nu} \int_0^\infty \frac{\cos(xt)}{(t^2 + z^2)^{\nu+\frac{1}{2}}} dt \quad \nu > -\frac{1}{2}, \quad x > 0, \quad z > 0, \quad (\text{S.162})$$

where  $K_\nu$  is the modified Bessel function of the second kind with order  $\nu$ . For  $\nu = p$ , this gives

$$A_n(r) = \int_{-\infty}^{\infty} \frac{\cos(n\pi y)}{(y^2 + r^2)^{p+\frac{1}{2}}} dy = \begin{cases} \frac{(p-1)!}{(2p-1)!!} \left(\frac{2}{r^2}\right)^p & (n=0) \\ \frac{2}{(2p-1)!!} \left(\frac{n\pi}{r}\right)^p K_p(n\pi r) & (n \geq 1) \end{cases}, \quad (\text{S.163})$$

as the Fourier coefficient. We restrict the definition of  $f(r, z)$  in Eq. (S.159) to strictly positive integers  $p = 1, 2, \dots$ , since the sum diverges when  $p = 0$  due to its asymptotically harmonic decay. This divergence stems entirely from the zeroth Fourier coefficient  $A_0(r)$ , which contains the term  $(p-1)!$  that diverges with  $p = 0$  under the usual definition of the Gamma function. In contrast, the higher Fourier modes  $A_n(r)$  for  $n \geq 1$  remain finite for all  $p \geq 0$ , as they are defined by convergent integrals through the Basset's formula (S.162). This mode-by-mode distinction proves helpful below when analyzing alternating series, for which the  $A_0$  contribution cancels identically and the Fourier expansion remains well-defined even at  $p = 0$ . Substituting the Fourier coefficients into Eq. (S.160) gives

$$\sum_{m=-\infty}^{\infty} \frac{1}{((2m+z)^2 + r^2)^{p+\frac{1}{2}}} = \frac{2}{(2p-1)!!} \frac{1}{r^p} \left[ \frac{(p-1)!}{4} \left(\frac{2}{r}\right)^p + \sum_{n=1}^{\infty} (n\pi)^p K_p(n\pi r) \cos(n\pi z) \right], \quad (\text{S.164})$$

as the relationship between the two representations, valid for any positive integer  $p$ . In this work, we frequently apply Eq. (S.164) for the case that  $z = 0$  and  $\cos(n\pi z) = 1$ .

We shall also encounter alternating series of the same structure as Eq. (S.159)

$$\sum_{m=-\infty}^{\infty} \frac{(-1)^m}{[(2m+z)^2 + r^2]^{p+\frac{1}{2}}},$$

where the period in  $z$  is 4. A similar analysis yields the identity

$$\sum_{m=-\infty}^{\infty} \frac{(-1)^m}{((2m+z)^2 + r^2)^{p+\frac{1}{2}}} = \frac{2}{(2p-1)!!} \frac{1}{r^p} \sum_{n=1}^{\infty} \left(\frac{2n-1}{2}\pi\right)^p K_p\left(\frac{2n-1}{2}\pi r\right) \cos\left(\frac{2n-1}{2}\pi z\right). \quad (\text{S.165})$$

This result is valid for any non-negative integer  $p$ , including  $p = 0$  (note that  $(-1)!! = 1$ ), due to the convergence of the original alternating series. Equation (S.165) can also be derived by subtracting two shifted copies of Eq. (S.164), one each for the positive and negative terms of the alternating series, i.e.  $[f(r/2, z/2) - f(r/2, z/2 - 1)]/2^{2p+1}$ .

While mathematically equivalent, the image-charge and spectral representations are useful in different limiting circumstances for  $r$ . From Eqs. (S.164) and (S.165), we see that when  $r \ll 1$ , the left-hand side at  $z = 0$  is dominated by the  $m = 0$  term, whereas the right-hand side still requires the full spectral sum. By contrast, for  $r \gg 1$ , every image charge contributes on the left-hand side, while on the right-hand side only the leading spectral term remains significant because  $K_p(x) \sim \sqrt{\pi/(2x)}e^{-x}$  as  $x \rightarrow \infty$ . Hence, the image-charge series is most convenient for small  $r$ , whereas the eigenfunction (Bessel) expansion is more efficient for large  $r$ .

Finally, we also consider a modification of Eq. (S.159), wherein a factor  $(2m+z)$  is added to the numerators in the sum. This is useful since partial fraction decomposition allows any image charge representation to be broken into terms of the above forms and those with an additional factor of  $(2m+z)$ . Such series are

odd in  $z$ , and therefore can be expanded in terms of Fourier sine series. Differentiating (S.164) and (S.165) with respect to  $z$  yields the following relations

$$\sum_{m=-\infty}^{\infty} \frac{2m+z}{((2m+z)^2+r^2)^{p+\frac{3}{2}}} = \frac{2}{(2p+1)!!} \frac{1}{r^p} \sum_{n=1}^{\infty} (n\pi)^{p+1} K_p(n\pi r) \sin(n\pi z) , \quad (\text{S.166})$$

$$\sum_{m=-\infty}^{\infty} \frac{(-1)^m(2m+z)}{((2m+z)^2+r^2)^{p+\frac{3}{2}}} = \frac{2}{(2p+1)!!} \frac{1}{r^p} \sum_{n=1}^{\infty} \left(\frac{2n-1}{2}\pi\right)^{p+1} K_p\left(\frac{2n-1}{2}\pi r\right) \sin\left(\frac{2n-1}{2}\pi z\right) . \quad (\text{S.167})$$

Again, it can be seen that the image charge solution and its corresponding eigenfunction expansion are useful to understand the small and large  $r$  limit, respectively.

## B. Hankel transforms of specific functions

Consider the function

$$\hat{F}_m(\hat{k}) = \left(-\frac{\hat{k}}{\tanh(\hat{k})}\right)^{m+1} , \quad (\text{S.168})$$

for an arbitrary non-negative integer  $m$ . Our goal is to compute the inverse Hankel transform of this function. We apply the partial fraction decomposition of  $1/\tanh(\hat{k})$  [12, (4.36.3)] to write

$$\hat{F}_m(\hat{k}) = \left(-1 - 2 \sum_{n=1}^{\infty} \frac{\hat{k}^2}{\hat{k}^2 + (n\pi)^2}\right)^{m+1} . \quad (\text{S.169})$$

Since  $-\hat{k}^2$  in the transform space corresponds to the radial Laplacian  $\hat{\nabla}^2$  in the real space, we have

$$\mathcal{H}[\hat{F}_m(\hat{k})](\hat{r}) = (\hat{\nabla}^2)^{m+1} \mathcal{H}\left[\left(\frac{1}{\hat{k}^2} + 2 \sum_{n=1}^{\infty} \frac{1}{\hat{k}^2 + (n\pi)^2}\right)^{m+1}\right](\hat{r}) , \quad (\text{S.170})$$

where  $\mathcal{H}$  is the inverse Hankel transform. Expanding the  $m+1$  power of the series and applying partial fraction decompositions yields

$$\left(\frac{1}{\hat{k}^2} + 2 \sum_{n=1}^{\infty} \frac{1}{\hat{k}^2 + (n\pi)^2}\right)^{m+1} = \sum_{l=0}^m \sum_{n=0}^{\infty} \frac{c_{n,l}}{(\hat{k}^2 + (n\pi)^2)^{l+1}} , \quad (\text{S.171})$$

where  $c_{n,l}$  is the coefficient of each term. The inverse transform of each term in the series is given by

$$\mathcal{H}\left[\frac{1}{(\hat{k}^2 + a^2)^{p+1}}\right](\hat{r}) = \left(\frac{\hat{r}}{2a}\right)^p \frac{K_p(a\hat{r})}{p!} , \quad (\text{S.172})$$

for  $a > 0$  [12, (10.22.46)]. When  $a = 0$  (i.e.  $n = 0$  terms in Eq. (S.171)), the Hankel transform corresponds to sharp variations near the origin  $\hat{r} = 0$  in the real space. Since we are interested in  $\hat{r} > 1$ , we may neglect the  $n = 0$  terms in the series:

$$\mathcal{H}[\hat{F}_m(\hat{k})](\hat{r}) = (\hat{\nabla}^2)^{m+1} \sum_{l=0}^m \sum_{n=1}^{\infty} c_{n,l} \left(\frac{\hat{r}}{2n\pi}\right)^l \frac{K_l(n\pi\hat{r})}{l!} . \quad (\text{S.173})$$

Next, we apply the Laplacian operator termwise by using

$$\hat{\nabla}^2(\hat{r}^p K_p(\hat{r})) = \hat{r}^p K_p(\hat{r}) - 2p\hat{r}^{p-1} K_{p-1}(\hat{r}) . \quad (\text{S.174})$$

Applying this recurrence relation repeatedly, we obtain

$$\left(\hat{\nabla}^2\right)^{m+1} \left(\hat{r}^l K_l(\hat{r})\right) = \sum_{q=0}^{\min\{l, m+1\}} (-1)^q q! 2^q \binom{m+1}{q} \binom{l}{q} \hat{r}^{l-q} K_{l-q}(\hat{r}) . \quad (\text{S.175})$$

Substituting this into Eq. (S.173) gives

$$\mathcal{H} \left[ \hat{F}_m(\hat{k}) \right] (\hat{r}) = \sum_{l=0}^m \sum_{n=1}^{\infty} \frac{c_{n,l}}{2^l (n\pi)^{2l} l!} (n\pi)^{2(m+1)} \sum_{q=0}^l (-1)^q q! 2^q \binom{m+1}{q} \binom{l}{q} (n\pi \hat{r})^{l-q} K_{l-q}(n\pi \hat{r}) . \quad (\text{S.176})$$

Further simplification by reindexing  $q \rightarrow l - q$  and  $l \rightarrow m - l$  yields

$$\mathcal{H} \left[ \hat{F}_m(\hat{k}) \right] (\hat{r}) = \sum_{n=1}^{\infty} \sum_{q=0}^m \frac{(-1)^{m-q} (n\pi \hat{r})^q K_q(n\pi \hat{r})}{q! 2^q} \sum_{l=0}^{m-q} c_{n, m-l} (n\pi)^{2(l+1)} (-1)^l \binom{m+1}{m-l-q} . \quad (\text{S.177})$$

Since Bessel functions scale asymptotically as  $K_q(x) \sim K_0(x)(1 + \mathcal{O}(x^{-1}))$  for all orders  $q$ , the dominant contribution at  $\hat{r} \gg 1$  in the series comes from the terms with the smallest  $n = 1$ , giving the slowest exponential decay, and the largest  $q = m$ , giving the highest power of  $\hat{r}$ . The leading order behavior in this limit is therefore given by

$$\mathcal{H} \left[ \hat{F}_m(\hat{k}) \right] (\hat{r}) \sim \frac{(\pi \hat{r})^m K_m(\pi \hat{r})}{m! 2^m} c_{1,m} \pi^2 \left( 1 + \mathcal{O}\left(\frac{1}{\hat{r}}\right) \right) . \quad (\text{S.178})$$

From Eq. (S.171), the coefficient  $c_{1,m}$  is associated with the factor  $(\hat{k}^2 + \pi^2)^{m+1}$ , which results from a single term in the expansion, giving  $c_{1,m} = 2^{m+1}$ . Substituting this gives the final result,

$$\mathcal{H} \left[ \left( -\frac{\hat{k}}{\tanh(\hat{k})} \right)^{m+1} \right] (\hat{r}) = \frac{2\pi^2 (\pi \hat{r})^m K_m(\pi \hat{r})}{m!} \left( 1 + \mathcal{O}\left(\frac{1}{\hat{r}}\right) \right) . \quad (\text{S.179})$$

Following a similar procedure, one obtains

$$\mathcal{H} \left[ \frac{\hat{k}}{\sinh(\hat{k})} \left( -\frac{\hat{k}}{\tanh(\hat{k})} \right)^m \right] (\hat{r}) = \frac{2\pi^2 (\pi \hat{r})^m K_m(\pi \hat{r})}{m!} \left( 1 + \mathcal{O}\left(\frac{1}{\hat{r}}\right) \right) , \quad (\text{S.180})$$

for  $\hat{r} \gg 1$  by representing  $1/\sinh(\hat{k})$  as a series [12, (4.36.5)].
